# Supplementary material for: Modular GPU Programming with Typed Perspectives
Source: arXiv:2511.11939 source file (2025-11-14)
Supplement: Supplementary file 1 [file appendix.pdf]

## A Complete Bundl Type System, Semantics, and Syntactic Soundness Proofs

### A.1 Basic Definitions

Hierarchy Levels  $h ::= \mathbf{Grid} | \mathbf{Block} | \mathbf{Thread}$

Memory Kinds  $l ::= \mathbf{Local} | \mathbf{Shared} | \mathbf{Global}$

Perspectives  $\pi : h \times \mathbb{N}$

Base Types  $b ::= \mathbf{bool} | \mathbf{int} | \mathbf{float}$

Types  $\tau ::= b | b[]^l | \mathbf{Fun}(\Gamma, \pi, m) | \mathbf{async} \tau$

Contexts  $\Gamma ::= \cdot | \Gamma, x :^\pi \tau$

Shared Memory Remaining  $m : \mathbb{N}$

Perspectives  $\pi$  are part of an algebra parameterized over some constant values  $T$  (the number of threads per block) and  $B$  (the number of blocks per grid). With these values, we have two isomorphisms:

$$(\mathbf{Block}, 1) \cong (\mathbf{Thread}, T)$$

and

$$(\mathbf{Grid}, 1) \cong (\mathbf{Block}, B)$$

The **group** and **split** operations of Prism allows us to move along this isomorphism, from left to right. For clarity, in Bundl we split these operations into three: a **split** operation that can split perspectives into multiple narrower ones, and a **destruct** operation that directly moves us along the isomorphism, and a **group** that divides our current perspective into equal sized parts.

Perspectives  $\pi$  are also lexicographically ordered in the obvious way.  $h$ s are ordered such that  $\mathbf{Thread} \leq \mathbf{Block} \leq \mathbf{Grid}$ , and  $(h_1, n_1) \leq (h_2, n_2)$  iff  $n_1 | n_2$  and  $h_1 \leq h_2$ .

We define scalar multiplication  $i \times h$  of natural numbers with  $h$ s:  $i \times (h, n) = (h, in)$ .

We also define division of perspectives and hierarchy levels of type  $\pi \times \pi \rightarrow \mathbb{N}$ .  $\mathbf{Grid}/\mathbf{Block} = B$  and  $\mathbf{Block}/\mathbf{Thread} = T$ . We lift this to perspectives like so:  $(h_1, n_1) / (h_2, n_2) = ((h_1/h_2) \cdot n_1) / n_2$ .

Lastly we define a partial  $\downarrow$  operator on  $h$ s such that  $\downarrow \mathbf{Block} = \mathbf{Thread}$  and  $\downarrow \mathbf{Grid} = \mathbf{Block}$ . Note that  $\downarrow \mathbf{Thread}$  is undefined. This operator lifts to  $\pi$ s whose second component is 1 and encodes the leftward component of the isomorphism above:  $\downarrow (\mathbf{Block}, 1) = (\mathbf{Thread}, T)$  and  $\downarrow (\mathbf{Grid}, 1) = (\mathbf{Block}, B)$ .

Note also that the presentation of these rules in the main body of the paper elide the  $m$  portion, which tracks the maximum amount of memory a given computation is allowed to use. In the full system presented here, both the typing rules and the operational semantics carry an additional piece of information tracking allocated memory.

### A.2 Complete Bundl Typing Rules

#### A.2.1 Expressions.

$$\frac{x :^\pi \tau \in \Gamma}{\Gamma \vdash^\pi x : \tau} \text{ T-Var} \quad \frac{}{\Gamma \vdash^\pi n : \mathbf{int}} \text{ T-Int} \quad \frac{}{\Gamma \vdash^\pi f : \mathbf{float}} \text{ T-Float}$$

$$\frac{}{\Gamma \vdash^\pi b : \mathbf{bool}} \text{ T-Bool} \quad \frac{\pi < (\mathbf{Grid}, 1)}{\Gamma \vdash^\pi \mathbf{partition\_id} : \mathbf{int}} \text{ T-Partition-Id}$$

$$\frac{\Gamma \vdash^{\pi'} e_1 : \tau[]^l \quad \Gamma \vdash^\pi e_2 : \mathbf{int} \quad l = \mathbf{Global} \text{ or } l = \mathbf{Local} \quad \pi \leq \pi'}{\Gamma \vdash^\pi e_1[e_2] : \tau} \text{ T-Arr-Access}$$

$$\begin{array}{c}
\frac{\Gamma \vdash^{\pi'} e_1 : \tau[]^{\text{Shared}} \quad \Gamma \vdash^{\pi} e_2 : \mathbf{int} \quad \pi \leq (\mathbf{Block}, 1) \quad \pi \leq \pi'}{\Gamma \vdash^{\pi} e_1[e_2] : \tau} \text{ T-Arr-Access-Shared} \\
\\
\frac{\Gamma \vdash^{\pi} e_1 : \mathbf{int} \quad \Gamma \vdash^{\pi} e_2 : \mathbf{int}}{\Gamma \vdash^{\pi} e_1 \mathbf{bop} e_2 : \mathbf{int}} \text{ T-Bop} \quad \frac{\Gamma \vdash^{\pi} e_1 : \mathbf{int} \quad \Gamma \vdash^{\pi} e_2 : \mathbf{int}}{\Gamma \vdash^{\pi} e_1 \mathbf{cmp} e_2 : \mathbf{bool}} \text{ T-Cmp} \\
\\
\text{A.2.2 Statements.} \\
\\
\frac{f : ^{\pi} \mathbf{Fun}(x_i : \tau_i, \pi, m') \in \Gamma \quad \Gamma \vdash^{\pi} e_i : \tau_i \quad m' \leq m}{\Gamma \vdash_m^{\pi} f(e_1, \dots, e_n)} \text{ T-Function-Call} \\
\\
\frac{\Gamma \vdash_m^{(h, n_1)} s_1 \quad \Gamma \vdash_m^{(h, n_2)} s_2 \quad n_1, n_2 \mathbf{align\ to\ } n}{\Gamma \vdash_m^{(h, n)} \mathbf{split}(n_1, n_2) \{s_1\} \{s_2\}} \text{ T-Split} \quad \frac{\Gamma \vdash_m^{\downarrow \pi} s}{\Gamma \vdash_m^{\pi} \mathbf{destruct\ in\ } s} \text{ T-Destruct} \\
\\
\frac{\Gamma \vdash_m^{(h, n)} s}{\Gamma \vdash_m^{(h, q \cdot n)} \mathbf{group\ } q \ s} \text{ T-Group} \quad \frac{x : ^{\pi'} \tau \in \Gamma \quad \Gamma \vdash^{\pi} e : \tau \quad \pi' \leq \pi}{\Gamma \vdash_m^{\pi} x = e} \text{ T-Assn} \\
\\
\frac{}{\Gamma \vdash_m^{\pi} \mathbf{init}_{\psi}} \text{ T-Sync-Init} \quad \frac{}{\Gamma \vdash_m^{\pi} \mathbf{dec}_{\psi}} \text{ T-Sync-Dec} \\
\\
\frac{}{\Gamma \vdash_m^{\pi} \mathbf{wait}_{\psi}} \text{ T-Sync-Wait} \quad \frac{}{\Gamma \vdash_m^{\pi} \mathbf{skip}} \text{ T-Skip} \quad \frac{n \leq m}{\Gamma \vdash_m^{\pi} \mathbf{free\ } n} \text{ T-Free} \\
\\
\frac{\Gamma \vdash^{\pi} e : \tau \quad \Gamma, x : ^{\pi'} \tau \vdash_m^{\pi} s \quad \pi' \leq \pi \quad \tau \text{ not an array type}}{\Gamma \vdash_m^{\pi} x : \tau \ @ \ \pi' = e \ \mathbf{in\ } s} \text{ T-Decl} \\
\\
\frac{\Gamma \vdash^{\pi'} e_1 : \tau[]^l \quad \Gamma \vdash^{\pi} e_2 : \mathbf{int} \quad \Gamma \vdash^{\pi} e_3 : \tau \quad l = \mathbf{Global} \text{ or } l = \mathbf{Local} \quad \pi' \leq \pi}{\Gamma \vdash_m^{\pi} e_1[e_2] = e_3} \text{ T-Arr-Assn} \\
\\
\frac{\Gamma \vdash^{\pi'} e_1 : \tau[]^{\text{Shared}} \quad \Gamma \vdash^{\pi} e_2 : \mathbf{int} \quad \Gamma \vdash^{\pi} e_3 : \tau \quad \pi \leq (\mathbf{Block}, 1) \quad \pi' \leq \pi}{\Gamma \vdash_m^{\pi} e_1[e_2] = e_3} \text{ T-Arr-Assn-Shared} \\
\\
\frac{\Gamma \vdash^{\pi} e : \mathbf{bool} \quad \Gamma \vdash_{m_1}^{\pi} s_1 \quad \Gamma \vdash_{m_2}^{\pi} s_2}{\Gamma \vdash_{\max(m_1, m_2)}^{\pi} \mathbf{if\ } e \text{ then } s_1 \text{ else } s_2} \text{ T-If} \\
\\
\frac{\Gamma \vdash^{\pi} e : \mathbf{bool} \quad \Gamma \vdash_m^{\pi} s}{\Gamma \vdash_m^{\pi} \mathbf{while\ } e \text{ do } s} \text{ T-While} \quad \frac{\Gamma \vdash_{m_1}^{\pi} s_1 \quad \Gamma \vdash_{m_2}^{\pi} s_2}{\Gamma \vdash_{\max(m_1, m_2)}^{\pi} s_1; s_2} \text{ T-Seq} \\
\\
\frac{\Gamma, x : ^{\pi} \tau[]^l \vdash_m^{\pi} s \quad l = \mathbf{Global} \text{ or } l = \mathbf{Local}}{\Gamma \vdash_{m+n \cdot \text{size}(\tau)}^{\pi} x := \mathbf{alloc\ } l \ \tau \ n \ \mathbf{in\ } s} \text{ T-Alloc} \\
\\
\frac{\Gamma, x : (\mathbf{Block}, 1) \tau[]^{\text{Shared}} \vdash_m^{\pi} s}{\Gamma \vdash_{m+n \cdot \text{size}(\tau)}^{(\mathbf{Block}, 1)} x := \mathbf{alloc\ Shared\ } \tau \ n \ \mathbf{in\ } s} \text{ T-Alloc-Shared} \\
\\
\frac{\Gamma, y : ^{(h, n/c)} \tau[]^l \vdash_m^{(h, n)} s \quad c | n \quad l \neq \mathbf{Local}}{\Gamma, x : ^{(h, n)} \tau[]^l \vdash_m^{(h, n)} \mathbf{partition}_{\psi} \ x \ \mathbf{into\ } y \ \mathbf{by\ } c \ \mathbf{in\ } s} \text{ T-Partition} \\
\\
\frac{\Gamma, y : ^{(h, n')} \tau[]^l \vdash_m^{(h, n')} s \quad n' \leq n \quad l \neq \mathbf{Local}}{\Gamma, x : ^{(h, n)} \tau[]^l \vdash_m^{(h, n)} \mathbf{claim}_{\psi} \ x \ \mathbf{into\ } y \ \mathbf{at\ } n' \ \mathbf{in\ } s} \text{ T-Claim}
\end{array}$$

$$\begin{array}{c}
\frac{\Gamma, y: \downarrow^\pi \tau[]^l \vdash_m^\pi s \quad l \neq \mathbf{Local}}{\Gamma, x: \pi \tau[]^l \vdash_m^\pi \mathbf{lower}_\psi x \text{ into } y \text{ in } s} \text{ T-Lower} \\
\\
\frac{\Gamma, y: (\mathbf{Thread}, 1) \mathbf{async} \tau[]^l \vdash_m^{(\mathbf{Thread}, 1)} s}{\Gamma, x: (\mathbf{Thread}, 1) \tau[]^l \vdash_m^{(\mathbf{Thread}, 1)} \mathbf{async\_partition}_\phi x \text{ into } y \text{ in } s} \text{ T-Async-Partition} \\
\\
\frac{}{\Gamma, x: (\mathbf{Thread}, 1) \mathbf{async} \tau[]^l, y: (\mathbf{Thread}, 1) \tau[]^{l'} \vdash_m^{(\mathbf{Thread}, 1)} \mathbf{async\_mempcy}(x, y)} \text{ T-Async-Memcpy} \\
\\
\frac{}{\Gamma, x: \pi \tau[]^l, y: \pi \tau[]^{l'} \vdash_m^\pi \mathbf{mempcy}(x, y)} \text{ T-Memcpy}
\end{array}$$

### A.3 Complete Bundl Semantics

#### A.3.1 Definitions.

Global Memory  $\Sigma ::= \cdot \mid \Sigma, n \mapsto^\pi v$

Shared Memory  $\sigma ::= \cdot \mid \sigma, n \mapsto^\pi v$

Local Memory  $\eta ::= \cdot \mid \eta, n \mapsto^\pi v$

Block Memory Map  $S ::= \forall n \in B, n \mapsto \sigma$

Thread Memory Map  $L ::= \forall n \in T, n \mapsto \eta$

Synchronization Map  $\Psi: \psi \rightarrow \mathbb{N} \rightarrow \mathbb{N}$

Deferred Computations Map  $\Phi: \phi \rightarrow \{s\}$

In real GPUs, thread IDs are only unique within their block. However, in this calculus for simplicity we assume thread IDs are global. One can convert back and forth between this abstracted notion of a thread ID and a block-unique ID via addition modulo  $T$ . That is,  $t_{\text{real}} = t_{\text{simplified}} \bmod T$  and  $t_{\text{simplified}} = t_{\text{real}} + b \cdot T$ .

By convention the names for local and shared and global memory do not conflict, as on the GPU they will be separate pointer spaces. Additionally, we freely interchange between using names for variables and integer locations.

In the main body of the paper, for simplicity we elide the synchronization map and the deferred computation map from the operational semantics, as our theorems do not make any guarantees about non-interference. However, as they are part of the full semantics, we include them here for completeness. By convention the synchronization and deferred computation maps are a total functions, initialized to map to  $\lambda\_0$  for  $\psi$ s and  $\lambda\_.$  for  $\phi$ s not explicitly initialize.

The shape of the judgment for a single thread is  $\eta, \sigma, \Sigma, t, b, p, \Psi \vdash_m^\pi s \rightsquigarrow s' \dashv_{m'} \eta', \sigma', \Sigma', \Psi'$ . The  $t$  here is the thread ID, the  $b$  is the block ID, and the  $p$  is the perspective ID. The last of these three is modified and managed by the rules for **split**, **group** and **destruct**, and tracks the relative position of the thread within a group. This semantics is in a small step style.

The shape of the judgment for expressions is  $\eta, \sigma, \Sigma \vdash_\pi^\pi e \Downarrow v$ . The two  $\pi$ s represent the ambient compute context (i.e., the context in which resources are being read), while  $\pi'$ , represents the target compute context (i.e., the compute context of the variable into which the result of the expression is going to be written. This is relevant for computing the value of **partition\_id**, which divides the two contexts. As a shorthand, we can divide a perspective by a scalar value like so:  $(h, n)/c = (h, n)/(h, c)$ .

The overall evaluation of a program is expressed as

$$L, S, \Sigma, P, \Psi, \Phi \rightsquigarrow L', S', \Sigma', P', \Psi', \Phi'.$$

In this judgment  $P$  serves as a *thread pool*, mapping pairs of thread and block IDs (which don't change) to statements and memory (which can be updated by stepping). One can think of  $P$  as tracking which program is running on each thread. This steps according to the following rule:

$$\frac{L(t), S(b), \Sigma, t, b, 0, \Psi, \Phi \vdash_m^{(\text{Grid}, 1)} s \rightsquigarrow s' \dashv_{m'} \eta', \sigma', \Sigma', \Psi', \Phi' \quad P(t, b) = (s, m)}{L, S, \Sigma, P, \Psi, \Phi \rightsquigarrow L[t \mapsto \eta'], S[b \mapsto \sigma'], \Sigma', P[(t, b) \mapsto (s', m')], \Psi', \Phi'} \text{ S-Program}$$

For simplicity of notation, we define an **update** operation that searches the three environments for the one that contains the variable being used (by convention, there is no conflict between the environments, as in reality they exist in three separate address spaces). We also define a similar **get** operation that retrieves a variable from memory, and a **rename** operation that remaps a variable with the same value but under a different name.

$$\mathbf{update}(\eta, \sigma, \Sigma, x, v) = (\eta[x \mapsto^\pi v], \sigma, \Sigma) \text{ when } x \in^\pi \eta$$

$$\mathbf{update}(\eta, \sigma, \Sigma, x, v) = (\eta, \sigma[x \mapsto^\pi v], \Sigma) \text{ when } x \in^\pi \sigma$$

$$\mathbf{update}(\eta, \sigma, \Sigma, x, v) = (\eta, \sigma, \Sigma[x \mapsto^\pi v]) \text{ when } x \in^\pi \Sigma$$

$$\mathbf{get}(\eta, \sigma, \Sigma, x) = \eta(x) \text{ when } x \in^\pi \eta$$

$$\mathbf{get}(\eta, \sigma, \Sigma, x) = \sigma(x) \text{ when } x \in^\pi \sigma$$

$$\mathbf{get}(\eta, \sigma, \Sigma, x) = \Sigma(x) \text{ when } x \in^\pi \Sigma$$

$$\mathbf{rename}(\eta, \sigma, \Sigma, x, y, \pi') = (\eta[y \mapsto^{\pi'} \eta(x)], \sigma, \Sigma) \text{ when } x \in^\pi \eta$$

$$\mathbf{rename}(\eta, \sigma, \Sigma, x, y, \pi') = (\eta, \sigma[y \mapsto^{\pi'} \sigma(x)], \Sigma) \text{ when } x \in^\pi \sigma$$

$$\mathbf{rename}(\eta, \sigma, \Sigma, x, y, \pi') = (\eta, \sigma, \Sigma[y \mapsto^{\pi'} \Sigma(x)]) \text{ when } x \in^\pi \Sigma$$

### A.3.2 Perspective Management Rules.

$$\frac{p < n_1 \quad n_1, n_2 \text{ align to } n \quad \eta, \sigma, \Sigma, t, b, p, \Psi, \Phi \vdash_m^{(h, n_1)} s_1 \rightsquigarrow s'_1 \dashv_{m'} \eta', \sigma', \Sigma', \Psi', \Phi'}{\eta, \sigma, \Sigma, t, b, p, \Psi, \Phi \vdash_m^{(h, n)} \mathbf{split}(n_1, n_2) \{s_1\} \{s_2\} \rightsquigarrow \mathbf{split}(n_1, n_2) \{s'_1\} \{s_2\} \dashv_{m'} \eta', \sigma', \Sigma', \Psi', \Phi'} \text{ S-Split-Left}$$

$$\frac{p < n_1 \quad n_1, n_2 \text{ align to } n}{\eta, \sigma, \Sigma, t, b, p, \Psi, \Phi \vdash_m^{(h, n)} \mathbf{split}(n_1, n_2) \{\mathbf{skip}\} \{s_2\} \rightsquigarrow \mathbf{skip} \dashv_m \eta, \sigma, \Sigma, \Psi, \Phi} \text{ S-Split-Left-Done}$$

$$\frac{p \geq n_1 \quad p < n_1 + n_2 \quad n_1, n_2 \text{ align to } n \quad \eta, \sigma, \Sigma, t, b, p - n_1, \Psi, \Phi \vdash_m^{(h, n_2)} s_2 \rightsquigarrow s'_2 \dashv_{m'} \eta', \sigma', \Sigma', \Psi', \Phi'}{\eta, \sigma, \Sigma, t, b, p, \Psi, \Phi \vdash_m^{(h, n)} \mathbf{split}(n_1, n_2) \{s_1\} \{s_2\} \rightsquigarrow \mathbf{split}(n_1, n_2) \{s_1\} \{s'_2\} \dashv_{m'} \eta', \sigma', \Sigma', \Psi', \Phi'} \text{ S-Split-Right}$$

$$\frac{p \geq n_1 \quad p < n_1 + n_2 \quad n_1, n_2 \text{ align to } n}{\eta, \sigma, \Sigma, t, b, p, \Psi, \Phi \vdash_m^{(h, n)} \mathbf{split}(n_1, n_2) \{s_1\} \{\mathbf{skip}\} \rightsquigarrow \mathbf{skip} \dashv_m \eta, \sigma, \Sigma, \Psi, \Phi} \text{ S-Split-Right-Done}$$

$$\frac{p \geq n_1 + n_2 \quad n_1, n_2 \text{ align to } n}{\eta, \sigma, \Sigma, t, b, p, \Psi, \Phi \vdash_m^{(h, n)} \mathbf{split}(n_1, n_2) \{s_1\} \{s_2\} \rightsquigarrow \mathbf{skip} \dashv_m \eta, \sigma, \Sigma, \Psi, \Phi} \text{ S-Split-None}$$

$$\frac{\eta, \sigma, \Sigma, t, b, t \text{ mod } T, \Psi, \Phi \vdash_m^{(\text{Thread}, T)} s \leadsto s' \dashv_{m'} \eta', \sigma', \Sigma', \Psi', \Phi'}{\eta, \sigma, \Sigma, t, b, 0, \Psi, \Phi \vdash_m^{(\text{Block}, 1)} \text{destruct in } s \leadsto \text{destruct in } s' \dashv_{m'} \eta', \sigma', \Sigma', \Psi', \Phi'} \quad \text{S-Destruct-Block}$$

$$\frac{\eta, \sigma, \Sigma, t, b, b \text{ mod } B, \Psi, \Phi \vdash_m^{(\text{Block}, B)} s \leadsto s' \dashv_{m'} \eta', \sigma', \Sigma', \Psi', \Phi'}{\eta, \sigma, \Sigma, t, b, 0, \Psi, \Phi \vdash_m^{(\text{Grid}, 1)} \text{destruct in } s \leadsto \text{destruct in } s' \dashv_{m'} \eta', \sigma', \Sigma', \Psi', \Phi'} \quad \text{S-Destruct-Grid}$$

$$\frac{}{\eta, \sigma, \Sigma, t, b, 0, \Psi, \Phi \vdash_m^\pi \text{destruct in skip} \leadsto \text{skip} \dashv_m \eta, \sigma, \Sigma, \Psi, \Phi} \quad \text{S-Destruct-Done}$$

$$\frac{\eta, \sigma, \Sigma, t, b, p \text{ mod } n, \Psi, \Phi \vdash_m^{(h, n)} s \leadsto s' \dashv_{m'} \eta', \sigma', \Sigma', \Psi', \Phi'}{\eta, \sigma, \Sigma, t, b, p, \Psi, \Phi \vdash_m^{(h, q \cdot n)} \text{group } q \leadsto \text{group } q \text{ } s' \dashv_{m'} \eta', \sigma', \Sigma', \Psi', \Phi'} \quad \text{S-Group}$$

$$\frac{}{\eta, \sigma, \Sigma, t, b, p, \Psi, \Phi \vdash_m^\pi \text{group } q \text{ skip} \leadsto \text{skip} \dashv_m \eta, \sigma, \Sigma, \Psi, \Phi} \quad \text{S-Group-Done}$$

**A.3.3 Thread Synchronization.** We define a **size** operation on perspectives to compute the size of a perspective (the number of individual compute resources sharing it). The operation is defined thusly:

$$\begin{aligned} \text{size}(\text{Thread}, n) &= n \\ \text{size}(\text{Block}, n) &= n \cdot T \\ \text{size}(\text{Grid}, n) &= n \cdot B \cdot T \end{aligned}$$

$$\frac{\Psi(\psi)(p) = 0}{\eta, \sigma, \Sigma, t, b, p, \Psi, \Phi \vdash_m^\pi \text{wait}_\psi \leadsto \text{skip} \dashv_m \eta, \sigma, \Sigma, \Psi, \Phi} \quad \text{S-Sync-Wait-Done}$$

$$\frac{\Psi(\psi)(p) \neq 0}{\eta, \sigma, \Sigma, t, b, p, \Psi, \Phi \vdash_m^\pi \text{wait}_\psi \leadsto \text{wait}_\psi \dashv_m \eta, \sigma, \Sigma, \Psi, \Phi} \quad \text{S-Sync-Wait-Spin}$$

$$\frac{\Psi' = \Psi(\psi)[p \mapsto \Psi(\psi)(p) - 1]}{\eta, \sigma, \Sigma, t, b, p, \Psi, \Phi \vdash_m^\pi \text{dec}_\psi \leadsto \text{skip} \dashv_m \eta, \sigma, \Sigma, \Psi', \Phi} \quad \text{S-Sync-Dec}$$

$$\frac{\Psi(\psi)(p) = 0 \quad \Psi' = \Psi(\psi)[p \mapsto \text{size}(\pi)]}{\eta, \sigma, \Sigma, t, b, p, \Psi, \Phi \vdash_m^\pi \text{init}_\psi \leadsto \text{skip} \dashv_m \eta, \sigma, \Sigma, \Psi', \Phi} \quad \text{S-Sync-Init-Zero}$$

$$\frac{\Psi(\psi)(p) \neq 0}{\eta, \sigma, \Sigma, t, b, p, \Psi, \Phi \vdash_m^\pi \text{init}_\psi \leadsto \text{skip} \dashv_m \eta, \sigma, \Sigma, \Psi, \Phi} \quad \text{S-Sync-Init-Nonzero}$$

**A.3.4 Asynchrony.**

$$\frac{\text{rename}(\eta, \sigma, \Sigma, x, y, (\text{Thread}, 1)), t, b, p, \Psi, \Phi \vdash_m^{(\text{Thread}, 1)} s \leadsto s' \dashv_{m'} \eta', \sigma', \Sigma', \Psi', \Phi'}{\eta, \sigma, \Sigma, t, b, p, \Psi, \Phi \vdash_{m'}^{(\text{Thread}, 1)} \text{async\_partition}_\phi x \text{ into } y \text{ in } s \leadsto \text{async\_partition}_\phi x \text{ into } y \text{ in } s' \dashv_{m'} \eta', \sigma', \Sigma', \Psi', \Phi'} \quad \text{S-Async-Partition-Congr}$$

$$\frac{\Phi = \Phi'[\phi \mapsto \Phi'(\phi) \cup \{s\}]}{\eta, \sigma, \Sigma, t, b, p, \Psi, \Phi \vdash_m^{(\text{Thread}, 1)} \text{async\_partition}_\phi x \text{ into } y \text{ in skip} \leadsto (\text{async\_partition}_\phi x \text{ into } y \text{ in } s) \dashv_m \eta, \sigma, \Sigma, \Psi, \Phi'} \quad \text{S-Async-Partition-Unwind}$$

$$\frac{\Phi(\phi) = \emptyset}{\eta, \sigma, \Sigma, t, b, p, \Psi, \Phi \vdash_m^{(\text{Thread}, 1)} \text{async\_partition}_{\phi} x \text{ into } y \text{ in skip} \rightsquigarrow \text{skip} \dashv_m \eta, \sigma, \Sigma, \Psi, \Phi} \text{ S-Async-Partition-Done}$$

$$\frac{}{\eta, \sigma, \Sigma, t, b, p, \Psi, \Phi \vdash_m^{(\text{Thread}, 1)} \text{async\_memcpy}(x, y) \rightsquigarrow \text{skip} \dashv_m \eta, \sigma, \Sigma, \Psi, \Phi[\phi \mapsto \Phi(\phi) \cup \{\text{memcpy}(x, y)\}]} \text{ S-Async-Memcpy}$$

$$\frac{(\eta', \sigma', \Sigma') = \text{update}(\eta, \sigma, \Sigma, x, \text{get}(\eta, \sigma, \Sigma, y))}{\eta, \sigma, \Sigma, t, b, p, \Psi, \Phi \vdash_m^{\pi} \text{memcpy}(x, y) \rightsquigarrow \text{skip} \dashv_m \eta', \sigma', \Sigma', \Psi, \Phi} \text{ S-Memcpy}$$

### A.3.5 Variables and Memory.

$$\frac{\eta, \sigma, \Sigma \vdash_{\pi'} e \Downarrow v \quad \pi' \leq \pi}{\eta, \sigma, \Sigma, t, b, p, \Psi, \Phi \vdash_m^{\pi} x : \tau \text{ @ } \pi' := e \text{ in } s \rightsquigarrow s \dashv_m \eta[x \mapsto^{\pi'} v], \sigma, \Sigma, \Psi, \Phi} \text{ S-Decl}$$

$$\frac{}{\eta, \sigma, \Sigma, t, b, p, \Psi, \Phi \vdash_m^{\pi} \text{free } n \dashv_{m-n} \eta, \sigma, \Sigma, \Psi, \Phi} \text{ S-Free}$$

$$\frac{\eta, \sigma, \Sigma, t, b, p, \Psi, \Phi \vdash_m^{\pi} x := \text{alloc Local } \tau \text{ n in } s \rightsquigarrow s; \text{ free } (n \cdot \text{size}(\tau)) \dashv_{m+n \cdot \text{size}(\tau)} \eta[x \mapsto^{\pi} \langle x, n \rangle], \sigma, \Sigma, \Psi, \Phi}{\eta, \sigma, \Sigma, t, b, p, \Psi, \Phi \vdash_m^{\pi} x := \text{alloc Local } \tau \text{ n in } s \rightsquigarrow s; \text{ free } (n \cdot \text{size}(\tau)) \dashv_{m+n \cdot \text{size}(\tau)} \eta[x \mapsto^{\pi} \langle x, n \rangle], \sigma, \Sigma, \Psi, \Phi} \text{ S-Alloc-Local}$$

$$\frac{\pi = (\text{Block}, 1)}{\eta, \sigma, \Sigma, t, b, p, \Psi, \Phi \vdash_m^{\pi} x := \text{alloc Shared } \tau \text{ n in } s \rightsquigarrow s; \text{ free } (n \cdot \text{size}(\tau)) \dashv_{m+n \cdot \text{size}(\tau)} \eta, \sigma[x \mapsto^{\pi} \langle x, n \rangle], \Sigma, \Psi, \Phi} \text{ S-Alloc-Shared}$$

$$\frac{}{\eta, \sigma, \Sigma, t, b, p, \Psi, \Phi \vdash_m^{\pi} x := \text{alloc Global } \tau \text{ n in } s \rightsquigarrow s; \text{ free } (n \cdot \text{size}(\tau)) \dashv_{m+n \cdot \text{size}(\tau)} \eta, \sigma, \Sigma[x \mapsto^{\pi} \langle x, n \rangle], \Psi, \Phi} \text{ S-Alloc-Global}$$

$$\frac{x \in \pi' \quad \eta, \sigma, \Sigma \quad \eta, \sigma, \Sigma \vdash_{\pi'} e \Downarrow v \quad (\eta', \sigma', \Sigma') = \text{update}(\eta, \sigma, \Sigma, x, v) \quad \pi' \leq \pi}{\eta, \sigma, \Sigma, t, b, p, \Psi, \Phi \vdash_m^{\pi} x = e \rightsquigarrow \text{skip} \dashv_m \eta', \sigma', \Sigma', \Psi, \Phi} \text{ S-Assn}$$

$$\frac{\eta, \sigma, \Sigma, t, b, p \vdash_{\pi} e_1 \Downarrow \langle l, n \rangle \quad i < n \quad \pi' \leq \pi \quad \eta, \sigma, \Sigma, t, b, p \vdash_{\pi} e_2 \Downarrow i \quad x \in \pi' \quad \eta, \sigma, \Sigma \quad \eta, \sigma, \Sigma \vdash_{\pi} e_3 \Downarrow v \quad (\eta', \sigma', \Sigma') = \text{update}(\eta, \sigma, \Sigma, l + i, v)}{\eta, \sigma, \Sigma, t, b, p, \Psi, \Phi \vdash_m^{\pi} e_1[e_2] = e_3 \rightsquigarrow \text{skip} \dashv_m \eta', \sigma', \Sigma', \Psi, \Phi} \text{ S-Arr-Assn}$$

$$\frac{s' = s[(y + c \cdot p) / y] \quad (\eta', \sigma', \Sigma') = \text{rename}(\eta, \sigma, \Sigma, x, y, \pi / c)}{\eta, \sigma, \Sigma, t, b, p, \Psi, \Phi \vdash_m^{\pi} \text{partition}/x \text{ ycs} \rightsquigarrow \text{init}_{\psi}; s'; \text{dec}_{\psi}; \text{wait}_{\psi} \dashv_m \eta', \sigma', \Sigma', \Psi, \Phi} \text{ S-Partition}$$

$$\frac{(\eta', \sigma', \Sigma') = \text{rename}(\eta, \sigma, \Sigma, x, y, (h, n_1))}{\eta, \sigma, \Sigma, t, b, p, \Psi, \Phi \vdash_m^{(h, n_1 + n_2)} \text{claim}_{\psi} x \text{ into } y \text{ at } n_1 \text{ in } s \rightsquigarrow \text{init}_{\psi}; \text{split}(n_1, n_2) \{s'\} \{\text{skip}\}; \text{dec}_{\psi}; \text{wait}_{\psi} \dashv_m \eta', \sigma', \Sigma', \Psi, \Phi} \text{ S-Claim}$$

$$\frac{(\eta', \sigma', \Sigma') = \text{rename}(\eta, \sigma, \Sigma, x, y, \downarrow \pi)}{\eta, \sigma, \Sigma, t, b, p, \Psi, \Phi \vdash_m^{\pi} \text{lower}_{\psi} x \text{ into } y \text{ in } s \rightsquigarrow \text{init}_{\psi}; s'; \text{dec}_{\psi}; \text{wait}_{\psi} \dashv_m \eta', \sigma', \Sigma', \Psi, \Phi} \text{ S-Lower}$$

### A.3.6 Control Flow.

$$\begin{array}{c}
\frac{\eta, \sigma, \Sigma \vdash_{\pi} e \Downarrow \text{true}}{\eta, \sigma, \Sigma, t, b, p, \Psi, \Phi \vdash_m^{\pi} \text{if } e \text{ then } s_1 \text{ else } s_2 \leadsto s_1 \dashv_m \eta, \sigma, \Sigma, \Psi, \Phi} \text{S-If-True} \\
\frac{\eta, \sigma, \Sigma \vdash_{\pi} e \Downarrow \text{false}}{\eta, \sigma, \Sigma, t, b, p, \Psi, \Phi \vdash_m^{\pi} \text{if } e \text{ then } s_1 \text{ else } s_2 \leadsto s_2 \dashv_m \eta, \sigma, \Sigma, \Psi, \Phi} \text{S-If-False} \\
\frac{}{\eta, \sigma, \Sigma, t, b, p, \Psi, \Phi \vdash_m^{\pi} \text{while } e \text{ do } s \leadsto \text{if } e \text{ then } (s; \text{while } e \text{ do } s) \text{ else skip} \dashv_m \eta, \sigma, \Sigma, \Psi, \Phi} \text{S-While} \\
\frac{\eta, \sigma, \Sigma, t, b, p, \Psi, \Phi \vdash_m^{\pi} s_1 \leadsto s'_1 \dashv_{m'}^{\pi'} \eta', \sigma', \Sigma', \Psi', \Phi'}{\eta, \sigma, \Sigma, t, b, p, \Psi, \Phi \vdash_m^{\pi} s_1; s_2 \leadsto s'_1; s_2 \dashv_{m'}^{\pi'} \eta', \sigma', \Sigma', \Psi', \Phi'} \text{S-Seq-First} \\
\frac{}{\eta, \sigma, \Sigma, t, b, p, \Psi, \Phi \vdash_m^{\pi} \text{skip}; s_2 \leadsto s_2 \dashv_m \eta, \sigma, \Sigma, \Psi, \Phi} \text{S-Seq-Done} \\
\frac{\Sigma(f) = \{[x_1 : \tau_1, \dots, x_n : \tau_n], s\} \quad \sigma, \Sigma \vdash_{\pi} e_i \Downarrow v_i \quad m' \leq m}{\eta, \sigma, \Sigma, t, b, p, \Psi, \Phi \vdash_m^{\pi} f(e_1, \dots, e_n) \leadsto s \dashv_m \eta[x_i \mapsto v_i], \sigma, \Sigma, \Psi, \Phi} \text{S-Function-Call}
\end{array}$$

### A.3.7 Expressions.

$$\begin{array}{c}
\frac{\pi < (\text{Grid}, 1) \quad \pi' \leq \pi}{\eta, \sigma, \Sigma \vdash_{\pi'} \text{partition\_id} \Downarrow \pi / \pi' - 1} \text{E-Partition-Id} \\
\frac{}{\eta, \sigma, \Sigma \vdash_{\pi'} x \Downarrow \text{get}(\eta, \sigma, \Sigma, x)} \text{E-Var} \\
\frac{\eta, \sigma, \Sigma \vdash_{\pi'} e_1 \Downarrow \langle l, n \rangle \quad \eta, \sigma, \Sigma \vdash_{\pi'} e_2 \Downarrow i \quad i < n \quad \pi' \leq \pi}{\eta, \sigma, \Sigma \vdash_{\pi'} e_1[e_2] \Downarrow \text{get}(\eta, \sigma, \Sigma, l+i)} \text{E-Arr-Access} \\
\frac{}{\eta, \sigma, \Sigma \vdash_{\pi'} \vdash n \Downarrow n} \text{E-Int} \quad \frac{}{\eta, \sigma, \Sigma \vdash_{\pi'} \vdash b \Downarrow b} \text{E-Bool} \\
\frac{\eta, \sigma, \Sigma \vdash_{\pi'} \vdash e_1 \Downarrow v_1 \quad \eta, \sigma, \Sigma \vdash_{\pi'} e_2 \Downarrow v_2 \quad v = v_1 \text{ bop } v_2}{\eta, \sigma, \Sigma \vdash_{\pi'} \vdash e_1 \text{ bop } e_2 \Downarrow v} \text{E-Bop} \\
\frac{\eta, \sigma, \Sigma \vdash_{\pi'} \vdash e_1 \Downarrow v_1 \quad \eta, \sigma, \Sigma \vdash_{\pi'} e_2 \Downarrow v_2 \quad v = v_1 \text{ cmp } v_2}{\eta, \sigma, \Sigma \vdash_{\pi'} \vdash e_1 \text{ cmp } e_2 \Downarrow v} \text{E-Cmp}
\end{array}$$

## A.4 Theorems and Proofs

Note that in this section we assume no out of bounds array accesses. In general Prism (and by extension Bundl) makes no guarantees about array out of bounds.

**A.4.1 More definitions.** As a premise to our type safety theorems, we need to assume we have a well-typed environment, written  $\Gamma \vdash \eta, \sigma, \Sigma$ . We define what this means inductively

$$\begin{array}{c}
\frac{}{\eta, \sigma, \Sigma \vdash n : \text{int}} \text{V-Int} \quad \frac{}{\eta, \sigma, \Sigma \vdash b : \text{bool}} \text{V-Bool} \quad \frac{}{\eta, \sigma, \Sigma \vdash f : \text{float}} \text{V-Float} \\
\frac{\forall i < n, \eta, \sigma, \Sigma \vdash \text{get}(\eta, \sigma, \Sigma, x+i) : \tau}{\eta, \sigma, \Sigma \vdash \langle x, n \rangle : \tau[]^l} \text{V-Array} \quad \frac{\Gamma, x_i : {}^{\pi} \tau_i \vdash_m^{\pi} s \quad \Gamma \vdash \cdot, \text{fns } \Sigma}{\eta, \sigma, \Sigma \vdash \{x_i : \tau_i, s\} : \text{Fun}(x_i : \tau_i, \pi, m)} \text{V-Function} \\
\frac{}{\cdot \vdash \eta, \sigma, \Sigma} \text{G-Empty} \quad \frac{\eta(x) = {}^{\pi} v \quad \eta, \sigma, \Sigma \vdash v : \text{int}}{\Gamma, x : {}^{\pi} \text{int} \vdash \eta, \sigma, \Sigma} \text{G-Int}
\end{array}$$

$$\begin{array}{c}
\frac{\eta(x) =^\pi v \quad \eta, \sigma, \Sigma \vdash v : \mathbf{bool}}{\Gamma, x : ^\pi \mathbf{bool} \vdash \eta, \sigma, \Sigma} \quad \mathbf{G-Bool} \qquad \frac{\eta(x) =^\pi v \quad \eta, \sigma, \Sigma \vdash v : \mathbf{float}}{\Gamma, x : ^\pi \mathbf{float} \vdash \eta, \sigma, \Sigma} \quad \mathbf{G-Float} \\
\\
\frac{\eta(x) =^\pi v \quad \eta, \sigma, \Sigma \vdash v : \tau[]}{\Gamma, x : ^\pi \tau[]^{\mathbf{Local}} \vdash \eta, \sigma, \Sigma} \quad \mathbf{G-Local} \qquad \frac{\sigma(x) =^\pi v \quad \eta, \sigma, \Sigma \vdash v : \tau[]}{\Gamma, x : ^\pi \tau[]^{\mathbf{Shared}} \vdash \eta, \sigma, \Sigma} \quad \mathbf{G-Shared} \\
\\
\frac{\Sigma(x) =^\pi v \quad \eta, \sigma, \Sigma \vdash v : \tau[]}{\Gamma, x : ^\pi \tau[]^{\mathbf{Global}} \vdash \eta, \sigma, \Sigma} \quad \mathbf{G-Global} \qquad \frac{\Sigma(x) =^\pi v \quad \eta, \sigma, \Sigma \vdash v : \mathbf{Fun}(\Gamma', \pi, m)}{\Gamma, x : ^\pi \mathbf{Fun}(\Gamma', \pi, m) \vdash \eta, \sigma, \Sigma} \quad \mathbf{G-Function}
\end{array}$$

We can prove a couple simple lemmas about well-typed environments under operations like **rename**, **update**, and **get**.

LEMMA A.1. (*Well-typed get*) If  $\Gamma \vdash \eta, \sigma, \Sigma$  and  $x : ^\pi \tau \in \Gamma$  then  $\eta, \sigma, \Sigma \vdash \mathbf{get}(\eta, \sigma, \Sigma, x) : \tau$ .

LEMMA A.2. (*Well-typed rename*) If  $\Gamma, x : ^\pi \tau \vdash \eta, \sigma, \Sigma$  then  $\Gamma, x : ^\pi \tau, y : ^{\pi'} \tau \vdash \mathbf{rename}(\eta, \sigma, \Sigma, x, y, \pi')$ .

LEMMA A.3. (*Well-typed update*) If  $\Gamma \vdash \eta, \sigma, \Sigma$  and  $\eta, \sigma, \Sigma \vdash v : \tau$  then  $\Gamma, x : ^\pi \tau \vdash \mathbf{update}(\eta, \sigma, \Sigma, x, v)$ .

We also define a well-formedness precondition on  $p$  with respect to  $\pi$ :

$$(h, n) \vdash p ::= p < n$$

We also define well-formedness for the async stack:

$$\Gamma \vdash \Phi ::= \forall \phi, s \in \Phi(\phi), \Gamma \vdash_m^{(\mathbf{Thread}, 1)} s$$

## A.5 Proofs

LEMMA A.4. (*Expression Safety*) If  $\Gamma \vdash^\pi e : \tau$  and  $\Gamma \vdash \eta, \sigma, \Sigma$  and  $\pi \vdash p$  and  $\pi' \leq \pi$ , then there is some  $v$  such that  $\eta, \sigma, \Sigma \vdash_{\pi'}^\pi e \Downarrow v$  and  $v : \tau$ .

PROOF. This proof proceeds by induction on the typing relation for expressions. Despite the fact that this property implies termination, we do not need a logical relation to prove it because the expression language is very simple.

The **T-Int**, **T-Float**, and **T-Bool** cases are trivial, using the rules **E-Int**, **E-Bool** and **E-Float** to compute values. In the case for **T-Partition-Id**, the  $\pi$  premises of the typing rules and our assumption that  $\pi' \leq \pi$  match the premises of the evaluation rule, so this rule is simple as well.

The cases for **T-Bop** and **T-Cmp** follow directly from the inductive hypotheses, assuming a valid and correctly implemented set of binary operators and comparators.

The only interesting cases are **T-Arr-Access** and **T-Arr-Access-Shared**.

In both cases our inductive hypotheses and inversion give us that  $\pi' \leq \pi$ , and  $e_1$  evaluates to a  $\langle x, n \rangle$ , and that all the values between  $x$  and  $x+n$  in the appropriate environment are typed at  $\tau$ . We also know that  $e_2$  evaluates to an integer  $i$ . We assume that all array accesses are in bounds, so  $i < l$ , which is sufficient to use the **E-Arr-Access** rule to complete this case, and the proof.  $\square$

LEMMA A.5. (*Expression Determinism*) If  $\eta, \sigma, \Sigma, t, b, p \vdash_{\pi'}^\pi e \Downarrow v_1$  and  $\eta, \sigma, \Sigma, t, b, p \vdash_{\pi'}^\pi e \Downarrow v_2$  then  $v_1 = v_2$ .

PROOF. Straightforward by induction on the semantic derivation.  $\square$

LEMMA A.6. (*Expression Well-Typedness*) If  $\Gamma \vdash_{\pi'}^\pi e : \tau$  and  $\Gamma \vdash \eta, \sigma, \Sigma$  and  $\pi \vdash p$ , and  $\eta, \sigma, \Sigma, t, b, p \vdash_{\pi'}^\pi e \Downarrow v$ , then  $v : \tau$ .

PROOF. By our expression safety lemma our well-typed expression must evaluate to a well-typed value  $v'$ . By our determinism lemma  $v'$  must be the same as  $v$ , so  $v$  is well-typed.  $\square$



LEMMA A.7. (*Statement Progress*) If  $\Gamma \vdash \eta, \sigma, \Sigma$  and  $\Gamma \vdash_m^\pi s$  and  $\pi \vdash p$ , then either  $s$  is **skip** or there is some  $s'$  such that  $\eta, \sigma, \Sigma, t, b, p, \Psi, \Phi \vdash_m^\pi s \leadsto s' \neg_{m''} \eta', \sigma', \Sigma, \Psi', \Phi'$

PROOF. This proceeds by induction on the typing derivation.

*Perspective Management Rules.*

- Case **T-Split**:

In this case we have by our assumption that  $\pi \vdash p$  that  $p < n$ . We also have that  $n_1, n_2$  **align to**  $n$ , so  $n_1 + n_2 \leq n$ . There are three cases to consider, then: when  $p < n_1$ , when  $p \geq n_1$  and  $p < n_1 + n_2$ , and when  $p \geq n_1 + n_2$ .

In the first case, we have by our inductive hypothesis that  $s$  is either **skip** or that it can step in an  $(h, n_1)$  context. In the former case we can use the **S-Split-Left-Done** rule and in the latter we can use the **S-Split-Left rule**.

The second case is almost symmetric. The only additional work we have to do is to argue that  $(h, n_2) \vdash p - n_1$ , or equivalently that  $p - n_1 < n_2$ . This, however, is immediate from our assumption that  $p < n_1 + n_2$ .

In the last case, we just use the **S-Split-None** rule to step to **skip**.

- Case **T-Destruct**

By our inductive hypothesis, we know that  $s$  can step at  $\downarrow \pi$  if  $\downarrow \pi \vdash p$ . The  $\downarrow$  operation is only defined at **(Block, 1)** or **(Grid, 1)**, so we only need to consider the cases where  $\pi$  is one of those.

In the former case  $p$  becomes  $t \bmod T$  while  $\downarrow \pi$  is **(Thread, T)**.  $t \bmod T < T$  for any  $t$  so this satisfies the requirement that  $\pi \vdash p$ , which lets us use our inductive hypothesis:  $s$  is either **skip** or can step. If it can step, we can use this to satisfy the premise of **S-Destruct-Block** to step in this case. If it is **skip**, then we use the rule **S-Destruct-Done** to step instead.

The latter case is the same, except using the fact that  $b \bmod B < B$  and the **S-Destruct-Grid** rule.

- Case **T-Group**

In this case we have by assumption that  $(h, q \cdot n) \vdash p$ , i.e., that  $p < q \cdot n$ .

In this case we have our IH that if  $(h, n) \vdash p'$  for some  $p'$ , then  $s$  is either **skip** or steps with  $(h, n)$  perspective with  $p'$  as our perspective ID.

We choose  $p'$  to be  $p \bmod n$ . This is always  $< n$ , so  $(h, n) \vdash p'$ . This lets us use our IH to get that  $s$  is either **skip** (in which case we can use the **S-Group-Done** rule to step) or itself steps, which lets us use the **S-Group** rule to step.

*Thread Synchronization Rules.*

- Case **T-Sync-Wait**

$\Psi(\psi)(p)$  is either zero or it is not. In the former case we use the **S-Sync-Wait-Done** rule and in the latter we use **S-Sync-Wait-Spin**.

- Case **T-Sync-Dec**

We use the **S-Sync-Dec** rule to step.

- Case **T-Sync-Init**

We use the **S-Sync-Init-Zero** or **S-Sync-Init-Nonzero** rules depending on whether  $\Psi(\psi)(p)$  is zero or not.

*Asynchrony Rules.*

- Case **T-Async-Partition**

In this case, we have via our IH that if  $\Gamma, y :^{(\text{Thread}, 1)} \text{async } \tau[] \vdash \eta', \sigma', \Sigma'$ , then we can either step  $s$  with **(Thread, 1)** perspective under environments  $\eta', \sigma'$ , and  $\Sigma'$ , or  $s$  is **skip**.

We have by assumption that  $\Gamma, x : (\text{Thread}, 1) \text{ async } \tau[]^l \vdash \eta, \sigma, \Sigma$ . By our environment renaming lemma, this gives us what we need to use our IH with  $(\eta', \sigma', \Sigma')$  as  $\text{rename}(\eta, \sigma, \Sigma, x, y, (\text{Thread}, 1))$ . Thus  $s$  either steps or is **skip**. In the former case we can step with **S-Async-Partition-Congr**, and in the latter we can use either **S-Async-Partition-Unwind** or **S-Async-Partition-Done** depending on whether  $\Phi(\phi)$  is empty or not.

- Case **T-Async-Memcpy**  
Immediate via use of the **S-Async-Memcpy** rule.
- Case **T-Memcpy**  
Immediate via use of the **S-Memcpy** rule.

#### Memory Rules.

- Case **T-Decl**  
Via our lemma about expression type safety and our hypothesis that  $e$  is well-typed, we obtain the premises necessary to use the **S-Decl** rule to step.
- Case **T-Arr-Assn**  
Each of  $e_1$ ,  $e_2$  and  $e_3$  must evaluate to a well-typed value by the expression type safety lemma. In particular, both  $e_1$  evaluates to some  $\langle l, n \rangle$  and  $e_2$  evaluates to some  $i$ . We assume all array accesses are in bounds, so this is sufficient to use the **S-Arr-Assn** rule to step.
- Case **T-Arr-Assn-Shared**  
Same as previous case.
- Case **T-Free**  
Trivial via the **S-Free** rule.
- Case **T-Partition**  
Trivial via the **S-Partition** rule.
- Case **T-Claim**  
Trivial via the **S-Claim** rule.
- Case **T-Lower**  
Trivial via the **S-Lower** rule.
- Case **T-Alloc**  
We assume that  $l$  is not **Shared**, so we can use the **S-Alloc-Local** or **S-Alloc-Global** rule, depending on whether  $l$  is **Local** or **Global**.
- Case **T-Alloc-Shared**  
Trivial via the **S-Alloc-Shared** rule.

#### Control Rules.

- Case **T-Skip**  
Trivial
- Case **T-While**  
Trivial, all while loops step via the **S-While** rule
- Case **T-If**  
By our proof of expression type safety, the expression  $e$  steps to either the boolean value true or false. We can thus use either the **S-If-True** or **S-If-False** rules to step.
- Case **T-Seq**  
In this case we know by our IH that  $s_1$  is either **skip** or can step. In the former case we use the **S-Seq-Done** rule and in the latter we use the **S-Seq-First** rule.
- Case **T-Function-Call**  
In this case we know by our expression safety lemma that each of the arguments will evaluate to a well-typed value. We also have by assumption that  $f$  has a function type, which by inversion

on the **V-Function** rule tells us that it is a closure type. Additionally our assumption that  $\Gamma \vdash \eta, \sigma, \Sigma$  tell us that  $\Sigma$  contains  $f$  at the same type that  $\Gamma$  does. These premises are sufficient to use the **S-Function-Call** rule.

□

LEMMA A.8. (*Statement Preservation*) If  $\Gamma \vdash \eta, \sigma, \Sigma$  and  $\Gamma \vdash_m^\pi s$  and  $\eta, \sigma, \Sigma, t, b, p, \Psi, \Phi \vdash_{m'}^\pi s \rightsquigarrow s' \dashv_{m''} \eta', \sigma', \Sigma, \Psi', \Phi'$  and  $\pi \vdash p$  and  $m \geq m'$  and  $\Gamma \vdash \Phi$ , then there is some  $\Gamma'$  such that  $\Gamma \subseteq \Gamma'$  and  $\Gamma' \vdash_m^\pi s'$  and  $\Gamma' \vdash \eta', \sigma', \Sigma'$  and  $m \geq m''$  and  $\Gamma' \vdash \Phi'$ .

PROOF. We proceed by induction on the derivation of  $\Gamma \vdash_m^\pi s$ .

*Perspective Management Rules.*

- Case **T-Split**

In this case we have by assumption that  $(h, n) \vdash p$ ,  $\Gamma \vdash \eta, \sigma, \Sigma$ , and  $\eta, \sigma, \Sigma, t, b, p, \Psi, \Phi \vdash_m^\pi \mathbf{split}(n_1, n_2) \{s_1\} \{s_2\} \rightsquigarrow s' \dashv_{m''} \eta', \sigma', \Sigma, \Psi', \Phi'$ . Our inductive hypotheses give us that if for any  $p$ , if  $(h, n_1) \vdash p$  and  $s_1$  steps with perspective ID  $p$ , or if  $(h, n_2) \vdash p$  and  $s_2$  steps with perspective ID  $p$  then their results are well typed.

By inversion on our semantic derivation, we are in one of 5 cases.

In the **S-Split-Left** case  $p < n_1$  and  $s_1$  steps to  $s'_1$ . This is sufficient to tell us that  $s'_1$  is well-typed and the output environments of that relation  $\eta', \sigma'$ , and  $\Sigma'$  are all well-typed by  $\Gamma' \supseteq \Gamma$ , and that the memory is properly bounded by the typing rules.

We can thus use the **T-Split-Left** rule to conclude that the result of this case is well-typed.

The **S-Split-Left-Done** rule is trivial via the **T-Skip** rule.

The **Right** cases are symmetric, with the observation that when  $p \geq n_1$  and  $p < n_1 + n_2$  then  $p - n_1 < n_2$ .

The last **S-Split-None** rule is trivial via the **T-Skip** rule.

- Case **T-Destruct**

In this case we have by assumption that  $\downarrow \pi$  is defined, so  $\pi$  is either (**Block**,1) or (**Grid**,1). We also assume that  $\eta, \sigma, \Sigma, t, b, p, \Psi, \Phi \vdash_{m'}^\pi \mathbf{destruct\ in} s \rightsquigarrow s' \dashv_{m''} \eta', \sigma', \Sigma, \Psi', \Phi'$ . We also have by our inductive hypothesis that for any  $p$  such that  $\downarrow \pi \vdash p$  and  $s''$  such that  $s$  steps to  $s''$  at  $p$ , then that step preserved well-typedness.

By inversion on the step relation, we are in one of three cases.

If the rule used **S-Destruct-Block**, then we know that  $s$  steps to  $s''$  and  $p$  is  $t \mathbf{mod} T$ . (**Thread**, $T$ )  $\vdash t \mathbf{mod} T$  for any  $t$ , so we can use our inductive hypothesis to conclude that the  $s''$  stepped to by  $s$  is well-typed, as are its environments and memory usage. The **T-Destruct** rule then gives us our desired goal.

The **S-Destruct-Grid** case proceeds similarly, while the **S-Destruct-Done** case is trivial.

- Case **T-Group**

In this case we have by assumption that

$\eta, \sigma, \Sigma, t, b, p, \Psi, \Phi \vdash_{m'}^{(h,q,n)} \mathbf{group} q s \rightsquigarrow s' \dashv_{m''} \eta', \sigma', \Sigma, \Psi', \Phi'$ . We have by our inductive hypothesis that  $s$  steps to  $s''$  at some perspective ID  $p'$  and  $(h, n) \vdash p'$ , then  $s''$  is well typed, as are the other outputs of that step.

By inversion on the step relation, we are in one of two cases. The **S-Group-Done** case is trivial, so we shall focus on the **S-Group** case. In this case we have that  $s$  steps to  $s''$  at perspective ID  $p \mathbf{mod} n$ . It is always the case that  $(h, n) \vdash p \mathbf{mod} n$  for any  $p$ , so we can use our inductive hypothesis to conclude that  $s''$  is well-typed, as are its output environments and memory usage. From there, it is a simple application of the **T-Group** rule to conclude that  $\mathbf{group} q s'$  is well-typed, and to finish the case.

*Thread Synchronization Rules.* These rules are all trivial: with one exception all thread synchronization primitives step to skip without changing environment or memory, and are thus obviously well-typed. **S-Sync-Wait-Spin** does not produce skip, but it steps to the same statement as we already assumed typechecks in the premise of the lemma, so is straightforward nonetheless.

If we wanted to say something about deadlock freedom we'd have more work here, but we aren't doing that, so these rules are easy.

*Asynchrony Rules.*

- **Case T-Async-Partition** In this case we have that  $s$  is well-typed in a context where  $x$  has been renamed into  $y$ , with  $(\mathbf{Thread}, 1)$  perspective. We also have that  $\Gamma, x : (\mathbf{Thread}, 1) \tau[]^l \vdash \eta, \sigma, \Sigma$  and  $\Gamma, x : (\mathbf{Thread}, 1) \tau[]^l \vdash \Phi$ .  
By inversion, we are in one of three cases.  
In the **S-Async-Partition-Done** case, we are done.  
In the **S-Async-Partition-Congr** case, our inductive hypothesis gives us that there is some  $\Gamma'$  such that  $\Gamma, y : (\mathbf{Thread}, 1) \mathbf{async} \tau[]^l \subseteq \Gamma'$  and  $\Gamma' \vdash \Phi'$  and  $\Gamma' \vdash \mathbf{rename}(\eta, \sigma, \Sigma, x, y, (\mathbf{Thread}, 1))$  via our well-typed renaming lemma. This lets us use the **T-Async-Partition** rule to check this case, with a choice of  $\Gamma'$  as  $\Gamma', x : (\mathbf{Thread}, 1) \tau[]^l$ .  
In the **S-Async-Partition-Unwind** case, our assumption that  $\Phi$  is well-typed tells us that  $\Gamma, y : (\mathbf{Thread}, 1) \vdash \{ (\mathbf{Thread}, 1)_m s$ . Thus, we can use the **T-Async-Partition** rule to type this case.
- **Case T-Async-Memcpy**  
In this case the statement and environment typing are trivial, we need only to show that the async stack remains well typed.  
In this case we have that  $x$  and  $y$  have the same type at  $(\mathbf{Thread}, 1)$ . This is sufficient for us to check  $x = y$  at  $(\mathbf{Thread}, 1)$ , meaning that adding that instruction to the stack maintains its well-typedness.
- **Case T-Memcpy**  
Immediate via use of the **S-Memcpy** rule. We just need to show that the environment remains well typed, which we know via our lemmas about **update** and **get**.

*Memory Rules.*

- **Case T-Decl**  
By inversion, we are using **S-Decl** rule for evaluation. Our well-typed expression lemma gives us that  $v$  is well-typed, so it follows from our assumptions and our lemmas about extending environments that the extended  $\eta$  and  $s$  are well-typed by  $\Gamma, x : \pi \tau$ .
- **Case T-Free**  
Trivial.
- **Case T-Alloc**  
By inversion we are either in the **S-Alloc-Local** or **S-Alloc-Global** rules. In either case, we assume that  $\Gamma, x : \pi \tau[]^l$  checks  $s$ , meaning we can use our extended environment lemmas and the **T-Seq** and **T-Free** rules to check these cases.
- **Case T-Alloc-Shared**  
Same as previous case.
- **Case T-Partition**  
In this case we have by assumption that  $\Gamma, y : (\mathbf{h}, n/c) \tau[]^l$  and  $l$  is not local and  $c$  divides  $n$ . By inversion on our step relation we must be in the **S-Partition** case, so we have  $\eta, \sigma, \Sigma, t, b, p, \Psi, \Phi \vdash_m^{\pi} \mathbf{partition}/xycs \rightsquigarrow \mathbf{init}_{\psi}; s'; \mathbf{dec}_{\psi}; \mathbf{wait}_{\psi} \dashv_m \eta', \sigma', \Sigma', \Psi, \Phi$  where  $s' = s[(y + c \cdot p)/y]$  and  $(\eta', \sigma', \Sigma') = \mathbf{rename}(\eta, \sigma, \Sigma, x, y, \pi/c)$ . Via our well-typed renaming lemma contexts we know that we can check the renamed environments in the extended environment  $\Gamma, y : \pi/c \tau[]^l, x : \pi$

$\tau[]^l$ , and this context is also sufficient to check  $s'$  (via a substitution-preserves-typing lemma that is obvious). Using the **T-Skip** rule this is exactly what we need to show to complete this case, as the thread sync primitives check trivially via their typing rules.

- Case **T-Claim**

Essentially the same as **T-Partition**.

- Case **T-Lower**

Essentially the same as **T-Partition**.

### Control Rules.

- Case **T-If**

We have by assumption that **if**  $e$  **then**  $s_1$  **else**  $s_2$  steps to some  $s'$ , and by inversion we know that either  $e$  evaluates to **true** and  $s'$  is  $s_1$ , or  $e$  evaluates to **false** and  $s'$  is  $s_2$ .

In either case, our inductive hypotheses is sufficient to tell us that these are well-typed. In particular, in both cases our IHs tell us that the amount of memory used by stepping each branch of the **if** is less than the amount of memory computed by the type system for each branch. Because the whole **if** expression checks using the greater of the memory usage of  $m_1$  or  $m_2$  (i.e., the memory usage on each branch), the resulting usage for the whole conditional is also bounded by the type system.

- Case **T-Skip**

Trivial: **skip** does not step

- Case **T-Seq**

In this case we have that  $s_1$  and  $s_2$  are both well-typed (with  $m_1$  memory and  $m_2$  memory respectively), and  $m = \max(m_1, m_2)$ . We also have by inversion that  $s_1$  either steps to **skip** or  $s'_1$ , and our inductive hypothesis tells us that  $s'_1$  is well-typed.

In the former case we can use the **S-Seq-Done** rule to trivially finish the case. In the latter, our IH allows us to finish the case, since  $m_1$  is always  $\leq \max(m_1, m_2)$

- Case **T-While**

By inversion, we have that

$$\begin{aligned} & \eta, \sigma, \Sigma, t, b, p, \Psi, \Phi \vdash_m^\pi \text{while } e \text{ do } s \\ & \leadsto \text{if } e \text{ then } (s; \text{while } e \text{ do } s) \text{ else skip} \dashv_m \eta, \sigma, \Sigma, \Psi, \Phi. \end{aligned}$$

We also have by assumption that  $e$  and  $s$  are well-typed. With this information, through use of the **T-If**, **T-Seq**, **T-While**, and **T-Skip** rules, we can conclude that the result of this rule is also well-typed.

- Case **T-Function-Call**

By inversion we have that

$$\begin{aligned} & \eta, \sigma, \Sigma, t, b, p, \Psi, \Phi \vdash_m^\pi f(e_1, \dots, e_n) \\ & \leadsto \text{call } s \text{ with } (x_i :^{\pi_i} \tau_i \mapsto v_i) @ \{\eta, \sigma, \Sigma, m'\} \dashv_m \eta, \sigma, \Sigma, \Psi, \Phi, \end{aligned}$$

and also that  $\Sigma(f) = \{[x_1 : \tau_1, \dots, x_n : \tau_n], s\}$ , and  $\eta, \sigma, \Sigma, t, b, p \vdash^\pi e_i \Downarrow v_i$ , and  $m' \leq m$ .

We also have from the premises of our case that  $f :^\pi \text{Fun}(x_1 :^{\pi_1} \tau_1, \dots, x_n :^{\pi_n} \tau_n, \pi, m') \in \Gamma$ , and  $\Gamma \vdash^\pi e_i : \tau_i$ , and  $m' \leq m$ .

Our lemma for expression well-typedness tells us that each  $v_i$  is a well-typed value, and our assumption that  $\Gamma \vdash \eta, \sigma, \Sigma$  tells us that  $\Sigma(f)$  is a well-typed function and thus that **fns**  $\Gamma, x_i :^{\pi_i} \tau_i \vdash_m^\pi s$ . We can take the union of this with  $\Gamma$  to produce  $\Gamma, x_i :^{\pi_i} \tau_i \vdash_{m'}^\pi s$ , which clearly checks  $s$  and the output environments.

□

## B Prism Programs

### B.1 Complete TF32 Matrix Multiplication

```

1765 @prism("device")
1766 @requires(thread[32])
1767 def simple_mma(a: ptr(const(float)) @ thread[32],
1768               b: ptr(const(float)) @ thread[32],
1769               c: ptr(float) @ thread[32]):
1770
1771     with group(thread[32]):
1772         stride : int @ thread[32] = 8
1773
1774         tid : int @ thread[1] = id()
1775
1776         regA: uint32_t[4] @ thread[1]
1777         row_a : int @ thread[1] = tid / 4
1778         col_a : int @ thread[1] = tid % 4
1779         offsetA : int @ thread[1] = row_a * stride + col_a
1780
1781         regA[0] = __float_as_uint(a[offsetA + 0])
1782         regA[1] = __float_as_uint(a[offsetA + 8 * stride]);
1783         regA[2] = __float_as_uint(a[offsetA + 4]);
1784         regA[3] = __float_as_uint(a[offsetA + 8 * stride + 4]);
1785
1786         regB: uint32_t[2] @ thread[1]
1787         row_b : int @ thread[1] = tid / 4
1788         col_b : int @ thread[1] = tid / 4
1789         offsetB : int @ thread[1] = row_b * stride + col_b
1790
1791         regB[0] = __float_as_uint(b[offsetB + 0])
1792         regB[1] = __float_as_uint(b[offsetB + 4 * stride])
1793
1794         regC: uint32_t[4] @ thread[1]
1795         regC[0] = 0
1796         regC[1] = 0
1797         regC[2] = 0
1798         regC[3] = 0
1799
1800         # Now do MMA!
1801         intrinsic.mma(
1802             regA[0], regA[1], regA[2], regA[3],
1803             regB[0], regB[1],
1804             regC[0], regC[1], regC[2], regC[3],
1805             out=[regC[0], regC[1], regC[2], regC[3]]
1806         )
1807
1808         row_c : uint32_t @ thread[1] = tid / 4
1809         col_c : int @ thread[1] = tid % 4
1810         offsetC : int @ thread[1] = row_c * stride + 2 * col_c
1811
1812         with partition(c, offset=offsetC, dimension=thread[1]) as c_thread:
1813             with group(thread[1]):
1814                 c_thread[0] += __uint_as_float(regC[0])
1815                 c_thread[1] += __uint_as_float(regC[1])
1816                 c_thread[8 * stride] += __uint_as_float(regC[2])
1817                 c_thread[8 * stride + 1] += __uint_as_float(regC[3])
1818
1819         return
1820
1821 @prism("global")
1822 @requires(grid[1], block[1], thread[32], smem=1280)
1823 def mmaTF32NaiveKernel(A: ptr(const(float)) @ grid[1],
1824                       B: ptr(const(float)) @ grid[1],
1825                       C: ptr(float) @ grid[1],
1826                       M : int @ grid[1],
1827                       N : int @ grid[1],
1828                       K : int @ grid[1]):
1829
1830     with group(grid[1]):
1831         MMA_N : constexpr(int) = 8
1832         MMA_K : constexpr(int) = 8
1833         MMA_M : constexpr(int) = 16
1834         K_tiles : const(int) = (K + MMA_K - 1) / MMA_K
1835
1836         num_blocks_n : const(int) @ grid[1] = (N + MMA_N - 1) / MMA_N
1837
1838         block_row : const(int) @ block[1] = id() / num_blocks_n
1839         block_col : const(int) @ block[1] = id() % num_blocks_n
1840
1841         warp_row: const(int) @ block[1] = block_row * MMA_M
1842         warp_col : const(int) @ block[1] = block_col * MMA_N
1843
1844         with claim(C, scope=block[1], offset= warp_row * N + warp_col) as C_blk:
1845             with group(block[1]):

```

```

1814 25 A_smem : shared(float[16 * 8]) @ block[1]
1815 26 B_smem : shared(float[8 * 8]) @ block[1]
1816 27 C_smem : shared(float[16 * 8]) @ block[1]
1817 28
1818 29 idx : int @ thread[1] = id() * 4
1819 30 with partition(C_smem, dimension=thread[1], offset=idx) as C_thrd:
1820 31     for i in range(0, 4, 1):
1821 32         with group(thread[1]):
1822 33             C_thrd[i] = 0
1823 34
1824 35 for i in range(0, K_tiles, 1):
1825 36     a_idx : int @ thread[1] = id() * 4
1826 37     # Sync point
1827 38     for j in range(0, 4, 1):
1828 39         flat_idx : int @ thread[1] = a_idx + j
1829 40         row : int @ thread[1] = flat_idx / MMA_K
1830 41         col : int @ thread[1] = flat_idx % MMA_K
1831 42         global_row : int @ thread[1] = warp_row + row
1832 43         global_col : int @ thread[1] = i * MMA_K + col
1833 44         with partition(A_smem, dimension=thread[1], offset= row * MMA_K + col) as A_smem_thrd:
1834 45             with group(thread[1]):
1835 46                 A_smem_thrd[0] = A[global_row * K + global_col]
1836 47
1837 48     b_idx : int @ thread[1] = id() * 2
1838 49     # Sync point
1839 50     for j in range(0, 2, 1):
1840 51         flat_idx_b : int @ thread[1] = b_idx + j
1841 52         row_b : int @ thread[1] = flat_idx_b / MMA_K
1842 53         col_b : int @ thread[1] = flat_idx_b % MMA_K
1843 54         global_row_b : int @ thread[1] = i * MMA_K + row_b
1844 55         global_col_b : int @ thread[1] = warp_col + col_b
1845 56         with partition(B_smem, dimension=thread[1], offset= row_b * MMA_K + col_b) as B_smem_thrd:
1846 57             with group(thread[1]):
1847 58                 B_smem_thrd[0] = B[global_row_b * N + global_col_b]
1848 59
1849 60     # Sync point
1850 61     with claim(C_smem, scope=thread[32], offset=0) as C_smem_warp:
1851 62         match split(thread):
1852 63             case 32:
1853 64                 simple_mma(A_smem, B_smem, C_smem_warp)
1854 65
1855 66 for j in range(0, 4, 1):
1856 67     flat_idx_c : int @ thread[1] = id() * 4 + j
1857 68     row_c : int @ thread[1] = flat_idx_c / MMA_K
1858 69     col_c : int @ thread[1] = flat_idx_c % MMA_K
1859 70     with partition(C_blk, dimension=thread[1], offset= row_c * N + col_c) as C_thrd:
1860 71         with group(thread[1]):
1861 72             C_thrd[0] = C_smem[row_c * MMA_N + col_c]
1862 73 return

```

## B.2 Different Matrix Multiplications Variants

```

1846 1 @prism("global")
1847 2 @requires(grid[1], block[1], thread[1], smem=49000)
1848 3 def my_sgemv_kernel_1(M : int @ grid[1],
1849 4     N : int @ grid[1],
1850 5     K : int @ grid[1],
1851 6     alpha : float @ grid[1],
1852 7     A: ptr(const(float)) @ grid[1],
1853 8     B: ptr(const(float)) @ grid[1],
1854 9     beta : float @ grid[1],
1855 10    C: ptr(float) @ grid[1],
1856 11    block_size : int @ grid[1]):
1857 12 with group(grid[1]):
1858 13     bid : int @ block[1] = id()
1859 14     with partition(C, dimension=block[1], offset=0) as C_blk:
1860 15         with group(block[1]):
1861 16             tid : int @ thread[1] = bid * block_size + id()
1862 17             with partition(C_blk, dimension=thread[1], offset=0) as C_thrd:
1863 18                 x : const(int) @ thread[1] = tid / N
1864 19                 y : const(int) @ thread[1] = tid % N
1865 20                 with group(thread[1]):
1866 21                     tmp : float @ thread[1] = 0
1867 22                     for i in range(0, K, 1):
1868 23                         tmp += A[x * K + i] * B[i * N + y]
1869 24                 C_thrd[x * N + y] = alpha * tmp + beta * C[x * N + y]
1870 25 return

```

```

1863 1 @prism("global")
1864 2 @requires(grid[1], block[1], thread[1], smem=49000)
1865 3 def my_sgemv_kernel_2(M : int @ grid[1],
1866 4                       N : int @ grid[1],
1867 5                       K : int @ grid[1],
1868 6                       alpha : float @ grid[1],
1869 7                       A: ptr(const(float)) @ grid[1],
1870 8                       B: ptr(const(float)) @ grid[1],
1871 9                       beta : float @ grid[1],
1872 10                      C: ptr(float) @ grid[1],
1873 11                      tile_size : int @ grid[1]):
1874 12     with group(grid[1]):
1875 13         global_tid: int @ thread[1] = id()
1876 14         total_elements : const(int) @ grid[1] = M * N
1877 15         num_tiles_per_row : const(int) @ grid[1] = (N + tile_size - 1) / tile_size
1878 16         tile_id : const(int) @ thread[1] = global_tid / (tile_size * tile_size)
1879 17         tile_row : const(int) @ thread[1] = tile_id / num_tiles_per_row
1880 18         tile_col : const(int) @ thread[1] = tile_id % num_tiles_per_row
1881 19         local_id : const(int) @ thread[1] = global_tid % (tile_size * tile_size)
1882 20         local_row : const(int) @ thread[1] = local_id / tile_size
1883 21         local_col : const(int) @ thread[1] = local_id % tile_size
1884 22         cRow : const(int) @ thread[1] = tile_row * tile_size + local_row
1885 23         cCol : const(int) @ thread[1] = tile_col * tile_size + local_col
1886 24         with partition(C, dimension=thread[1], offset=cRow * N + cCol) as C_thrd:
1887 25             with group(thread[1]):
1888 26                 if global_tid < total_elements:
1889 27                     if cRow < M and cCol < N:
1890 28                         tmp : float @ thread[1] = 0
1891 29                         for i in range(0, K, 1):
1892 30                             tmp += A[cRow * K + i] * B[i * N + cCol]
1893 31                         C_thrd[0] = alpha * tmp + beta * C_thrd[0]
1894 32
1895 33     return
1896 34

```



```

1912 1 @prism("global")
1913 2 @attr("__launch_bounds__((BM * BN) / (TM * TN), 1)")
1914 3 @template(["BM", c_int),
1915 4           ("BN", c_int),
1916 5           ("BK", c_int),
1917 6           ("TM", c_int),
1918 7           ("TN", c_int)])
1919 8 @requires(grid[1], block[1], thread[1], smem=49000)
1920 9 def my_sgemv_kernel_3(M : int @ grid[1],
1921 10                      N : int @ grid[1],
1922 11                      K : int @ grid[1],
1923 12                      alpha : float @ grid[1],
1924 13                      A: ptr(const(float)) @ grid[1],
1925 14                      B: ptr(const(float)) @ grid[1],
1926 15                      beta : float @ grid[1],
1927 16                      C: ptr(float) @ grid[1],
1928 17                      num_blocks_N : int @ grid[1]):
1929 18     with group(grid[1]):
1930 19         cRow : const(int) @ block[1] = id() / num_blocks_N
1931 20         cCol : const(int) @ block[1] = id() % num_blocks_N
1932 21         totalResultsBlocktile: const(uint) @ grid[1] = BM * BN
1933 22         numThreadsBlocktile: const(uint) @ grid[1] = totalResultsBlocktile / (TM * TN)
1934 23         with partition(C, dimension=block[1], offset = cRow * BM * N + cCol * BN) as C_blk:
1935 24             with partition(A, dimension=block[1], offset = cRow * BM * K) as A_blk:
1936 25                 with partition(B, dimension=block[1], offset = cCol * BN) as B_blk:
1937 26                     with group(block[1]):
1938 27                         As : shared(float[128 * 8]) @ block[1]
1939 28                         Bs : shared(float[128 * 8]) @ block[1]
1940 29                         threadRow : const(int) @ thread[1] = id() / (BN / TN)
1941 30                         threadCol : const(int) @ thread[1] = id() % (BN / TN)
1942 31
1943 32                         innerRowA : const(int) @ thread[1] = id() / BK
1944 33                         innerColA : const(int) @ thread[1] = id() % BK
1945 34                         strideA : const(int) @ thread[1] = numThreadsBlocktile / BK
1946 35
1947 36                         innerRowB : const(int) @ thread[1] = id() / BN
1948 37                         innerColB : const(int) @ thread[1] = id() % BN
1949 38                         strideB : const(int) @ thread[1] = numThreadsBlocktile / BN
1950 39
1951 40                         threadResults : float[64] @ thread[1] = { 0 }
1952 41                         regM : float[8] @ thread[1] = { 0 } # Need to go add the {}
1953 42                         regN : float[8] @ thread[1] = { 0 }
1954 43
1955 44                         i : int @ thread[1] = 0
1956 45
1957 46                         for bkIdx in range(0, K, BK):
1958 47
1959 48                             with partition(As, dimension=thread[1], offset = 0) as As_thrd:
1960 49                                 with partition(Bs, dimension=thread[1], offset = 0) as Bs_thrd:
1961 50                                     with group(thread[1]):
1962 51                                         for loadOffset in range(0, BM, strideA):
1963 52                                             As_thrd[(innerRowA + loadOffset) * BK + innerColA] = \
1964 53                                                 A_blk[i * BK + (innerRowA + loadOffset) * K + innerColA]
1965 54
1966 55                                         for loadOffset in range(0, BK, strideB):
1967 56                                             Bs_thrd[(innerRowB + loadOffset) * BN + innerColB] = \
1968 57                                                 B_blk[(i * BK * N) + (innerRowB + loadOffset) * N + innerColB]
1969 58
1970 59                                             i += 1
1971 60
1972 61                                         for dotIdx in range(0, BK, 1):
1973 62                                             for i in range(0, TN, 1):
1974 63                                                 regM[i] = As[(threadRow * TM + i) * BK + dotIdx]
1975 64                                             for i in range(0, TN, 1):
1976 65                                                 regN[i] = Bs[dotIdx * BN + threadCol * TN + i]
1977 66                                         for resIdxM in range(0, TM, 1):
1978 67                                             for resIdxN in range(0, TN, 1):
1979 68                                                 threadResults[resIdxM * TN + resIdxN] += regM[resIdxM] * regN[resIdxN]
1980 69
1981 70                                         for resIdxM in range(0, TM, 1):
1982 71                                             for resIdxN in range(0, TN, 1):
1983 72                                                 with partition(C_blk, dimension=thread[1], offset = (threadRow * TM + resIdxM) * N + threadCol * TN +
1984 73                                                     resIdxN) as C_thrd:
1985 74                                                     with group(thread[1]):
1986 75                                                         C_thrd[0] = alpha * threadResults[resIdxM * TN + resIdxN] + beta * C_blk[(threadRow * TM + resIdxM) *
1987 76                                                         N + threadCol * TN + resIdxN]
1988 77
1989 78     return

```

```

1661 1 @prism("global")
1662 2 @attr("__launch_bounds__((BM * BN) / (TM * TN), 1)")
1663 3 @template[["BM", c_int),
1664 4 ("BN", c_int),
1665 5 ("BK", c_int),
1666 6 ("TM", c_int),
1667 7 ("TN", c_int)]]
1668 8 @requires(grid[1], block[1], thread[1], smem=49000)
1669 9 def my_sgemv_kernel_4(M : int @ grid[1],
1670 10 N : int @ grid[1],
1671 11 K : int @ grid[1],
1672 12 alpha : float @ grid[1],
1673 13 A: ptr(float) @ grid[1],
1674 14 B: ptr(float) @ grid[1],
1675 15 beta : float @ grid[1],
1676 16 C: ptr(float) @ grid[1],
1677 17 num_blocks_N : int @ grid[1]):
1678 18 with group(grid[1]):
1679 19     cRow : const(int) @ block[1] = id() / num_blocks_N
1680 20     cCol : const(int) @ block[1] = id() % num_blocks_N
1681 21     totalResultsBlocktile: const(uint) @ grid[1] = BM * BN
1682 22     numThreadsBlocktile: const(uint) @ grid[1] = totalResultsBlocktile / (TM * TN)
1683 23     with partition(C, dimension=block[1], offset = cRow * BM * N + cCol * BN) as C_blk:
1684 24         with partition(A, dimension=block[1], offset = cRow * BM * K) as A_blk:
1685 25             with partition(B, dimension=block[1], offset = cCol * BN) as B_blk:
1686 26                 with group(block[1]):
1687 27                     As : shared(float[128 * 8]) @ block[1]
1688 28                     Bs : shared(float[128 * 8]) @ block[1]
1689 29                     threadRow : const(int) @ thread[1] = id() / (BN / TN)
1690 30                     threadCol : const(int) @ thread[1] = id() % (BN / TN)
1691 31
1692 32                     innerRowA : const(int) @ thread[1] = id() / (BK / 4)
1693 33                     innerColA : const(int) @ thread[1] = id() % (BK / 4)
1694 34                     strideA : const(int) @ thread[1] = numThreadsBlocktile / BK
1695 35
1696 36                     innerRowB : const(int) @ thread[1] = id() / (BN / 4)
1697 37                     innerColB : const(int) @ thread[1] = id() % (BN / 4)
1698 38                     strideB : const(int) @ thread[1] = numThreadsBlocktile / BN
1699 39
1700 40                     threadResults : float[64] @ thread[1] = { 0 }
1701 41                     regM : float[8] @ thread[1] = { 0 } # Need to go add the {}
1702 42                     regN : float[8] @ thread[1] = { 0 }
1703 43
1704 44                     i : int @ thread[1] = 0
1705 45
1706 46                     for bkIdx in range(0, K, BK):
1707 47
1708 48                         with partition(As, dimension=thread[1], offset = 0) as As_thrd:
1709 49                             with partition(Bs, dimension=thread[1], offset = 0) as Bs_thrd:
1710 50                                 with group(thread[1]):
1711 51
1712 52                                     tmp : float4 @ thread[1] = float4_cast(A_blk[i * BK + innerRowA * K + innerColA * 4])
1713 53                                     As_thrd[innerColA * 4 + 0] * BM + innerRowA] = tmp.x
1714 54                                     As_thrd[innerColA * 4 + 1] * BM + innerRowA] = tmp.y
1715 55                                     As_thrd[innerColA * 4 + 2] * BM + innerRowA] = tmp.z
1716 56                                     As_thrd[innerColA * 4 + 3] * BM + innerRowA] = tmp.w
1717 57
1718 58                                     i += 1
1719 59
1720 60                                 for dotIdx in range(0, BK, 1):
1721 61                                     for i in range(0, TN, 1):
1722 62                                         regM[i] = As[dotIdx * BM + threadRow * TM + i]
1723 63                                     for i in range(0, TN, 1):
1724 64                                         regN[i] = Bs[dotIdx * BN + threadCol * TN + i]
1725 65                                     for resIdxM in range(0, TM, 1):
1726 66                                         for resIdxN in range(0, TN, 1):
1727 67                                             threadResults[resIdxM * TN + resIdxN] += regM[resIdxM] * regN[resIdxN]
1728 68
1729 69                                 for resIdxM in range(0, TM, 1):
1730 70                                     for resIdxN in range(0, TN, 4):
1731 71                                         with partition(C_blk, dimension=thread[1], offset = (threadRow * TM + resIdxM) * N + threadCol * TN +
1732 72                                             resIdxN) as C_thrd:
1733 73                                             with group(thread[1]):
1734 74                                                 temp : float4 = float4_cast(C_thrd[0])
1735 75                                                 temp.x = alpha * threadResults[resIdxM * TN + resIdxN] + beta * temp.x
1736 76                                                 temp.y = alpha * threadResults[resIdxM * TN + resIdxN + 1] + beta * temp.y
1737 77                                                 temp.z = alpha * threadResults[resIdxM * TN + resIdxN + 2] + beta * temp.z
1738 78                                                 temp.w = alpha * threadResults[resIdxM * TN + resIdxN + 3] + beta * temp.w
1739 79                                                 float4_cast[C_thrd[0]] = temp
1740 80
1741 81                                 return

```

```

2010 1 @prism("global")
2011 2 @attr("__launch_bounds__(NUM_THREADS)")
2012 3 @template([("BM", c_int),
2013 4 ("BN", c_int),
2014 5 ("BK", c_int),
2015 6 ("WM", c_int),
2016 7 ("WN", c_int),
2017 8 ("WNITER", c_int),
2018 9 ("TM", c_int),
2019 10 ("TN", c_int),
2020 11 ("NUM_THREADS", c_int),
2021 12 ])
2022 13 @requires(grid[1], block[1], warp[1], smem=49000)
2023 14 def my_sgemv_kernel_5(M : int @ grid[1],
2024 15 N : int @ grid[1],
2025 16 K : int @ grid[1],
2026 17 alpha : float @ grid[1],
2027 18 A : ptr(float) @ grid[1],
2028 19 B : ptr(float) @ grid[1],
2029 20 beta : float @ grid[1],
2030 21 C : ptr(float) @ grid[1],
2031 22 num_blocks_N : int @ grid[1]):
2032 23
2033 24 with group(grid[1]):
2034 25   cRow : const(int) @ block[1] = id() / num_blocks_N
2035 26   cCol : const(int) @ block[1] = id() % num_blocks_N
2036 27
2037 28   WMITER : constexpr(uint) @ grid[1] = (WM * WN) / (WARPSIZE * TM * TN * WNITER)
2038 29   WSUBM : constexpr(uint) @ grid[1] = WM / WMITER
2039 30   WSUBN : constexpr(uint) @ grid[1] = WN / WNITER
2040 31
2041 32   rowStrideA : constexpr(int) @ grid[1] = (NUM_THREADS * 4) / BK
2042 33   rowStrideB : constexpr(int) @ grid[1] = NUM_THREADS / (BN / 4)
2043 34   with partition(C, dimension=block[1], offset = cRow * BM * N + cCol * BN) as C_blk:
2044 35     with partition(A, dimension=block[1], offset = cRow * BM * K) as A_blk:
2045 36       with partition(B, dimension=block[1], offset = cCol * BN) as B_blk:
2046 37         with group(block[1]):
2047 38           warpIdx : const(uint) @ thread[32] = id()
2048 39           warpCol : const(uint) @ thread[32] = warpIdx % (BN / WN)
2049 40           warpRow : const(uint) @ thread[32] = warpIdx / (BN / WN)
2050 41           As : shared(float[128 * 16]) @ block[1]
2051 42           Bs : shared(float[128 * 16]) @ block[1]
2052 43
2053 44           innerRowA : const(int) @ thread[1] = id() / (BK / 4)
2054 45           innerColA : const(int) @ thread[1] = id() % (BK / 4)
2055 46
2056 47           innerRowB : const(int) @ thread[1] = id() / (BN / 4)
2057 48           innerColB : const(int) @ thread[1] = id() % (BN / 4)
2058 49
2059 50           threadResults : float[128] @ thread[1] = { 0 }
2060 51           regM : float[8] @ thread[1] = { 0 } # Need to go add the {}
2061 52           regN : float[16] @ thread[1] = { 0 }
2062 53           j : int @ block[1] = 0
2063 54           for bkIdx in range(0, K, BK):
2064 55             with partition(A_blk, dimension=block[1], offset = j * BK) as A_offset:
2065 56               with partition(B_blk, dimension=block[1], offset = j * BK * N) as B_offset:
2066 57                 loadFromGmem_our(N, K, A_offset, B_offset, As, Bs, template=[BM, BN, BK, rowStrideA, rowStrideB])
2067 58                 processFromSmem_our(regM, regN, threadResults, As, Bs, warpRow, warpCol, template=[BM, BN, BK, WM, WN,
2068 59                 ↪ WMITER, WNITER, WSUBM, WSUBN, TM, TN])
2069 60                 j+=1
2070 61                 pass
2071 62
2072 63           with partition(C_blk, dimension=warp[1], offset = warpRow * WM * N + warpCol * WN) as C_warp:
2073 64             with group(warp[1]):
2074 65               threadIdxInWarp : int @ thread[1] = id()
2075 66               threadColInWarp : const(uint) @ thread[1] = threadIdxInWarp % (WSUBN / TN)
2076 67               threadRowInWarp : const(uint) @ thread[1] = threadIdxInWarp / (WSUBN / TN)
2077 68
2078 69               for wSubRowIdx in range(0, WMITER, 1):
2079 70                 for wSubColIdx in range(0, WNITER, 1):
2080 71                   with partition(C_warp, dimension=thread[1], offset = (wSubRowIdx * WSUBM) * N + wSubColIdx * WSUBN)
2081 72                   ↪ as C_interim:
2082 73                     for resIdxM in range(0, TM, 1):
2083 74                       for resIdxN in range(0, TN, 4):
2084 75                         with group(thread[1]):
2085 76                           tmp : float4 @ thread[1] = float4_cast(C_interim[(threadRowInWarp * TM + resIdxM) * N +
2086 77                           ↪ threadColInWarp * TN + resIdxN])
2087 78                           i : const(int) @ thread[1] = (wSubRowIdx * TM + resIdxM) * (WNITER * TN) + wSubColIdx * TN
2088 79                           ↪ + resIdxN
2089 80                           tmp.x = alpha * threadResults[i + 0] + beta * tmp.x
2090 81                           tmp.y = alpha * threadResults[i + 1] + beta * tmp.y
2091 82                           tmp.z = alpha * threadResults[i + 2] + beta * tmp.z
2092 83                           tmp.w = alpha * threadResults[i + 3] + beta * tmp.w
2093 84                           float4_cast[C_interim[(threadRowInWarp * TM + resIdxM) * N + threadColInWarp * TN +
2094 85                           ↪ resIdxN]] = tmp
2095 86
2096 87 return

```

### B.3 Single-Pass Parallel Prefix Scan with Decoupled Look-Back

```

2059
2060 1 @prism("global")
2061 2 @requires(grid[1], thread[1])
2062 3 def add_m_thread(x: ptr(const(c_int)) @ grid[1],
2063 4 y: ptr(c_int) @ grid[1],
2064 5 m: uint32_t @ grid[1]):
2065 6 with group(grid[1]):
2066 7 tid : uint32_t @ thread[1] = id()
2067 8 with partition(x, offset=tid, dimension=thread[1]) as x_thread:
2068 9 with partition(y, offset=tid, dimension=thread[1]) as y_thread:
2069 10 with group(thread[1]):
2070 11 y_thread[0] = x_thread[0] + m
2071 12 return
2072 13
2073 14 # WORK_PER_BLOCK = (8192 * 2)
2074 15 # WARPS_PER_BLOCK = 16
2075 16 # WARPS_PASS_CNT = (8192 * 2) / (16 * 32) = 32
2076 17 # WARP_ENDS = (8192 * 2) / 32 = 512
2077 18
2078 19 @prism("device")
2079 20 @requires(thread[1])
2080 21 def shfl_up_sync_wrapper(val : uint32_t @ thread[1], delta : uint32_t @ thread[1]):
2081 22 pass
2082 23
2083 24 @prism("device")
2084 25 @requires(block[1], warp[16])
2085 26 def scan_warps(x : ptr(uint32_t) @ block[1], x_shmem : ptr(uint32_t) @ block[1]):
2086 27 with group(block[1]):
2087 28 for i in range(0, (8192 * 2) / (16 * 32)):
2088 29 warp_id : uint32_t @ warp[1] = id()
2089 30 with partition(x, offset = (warp_id + i * 16) * 32, dimension = warp[1]) as x_warp:
2090 31 with partition(x_shmem, offset = (warp_id + i * 16) * 32, dimension = warp[1]) as x_shmem_warp:
2091 32 with group(warp[1]):
2092 33 thread_id : uint32_t @ thread[1] = id()
2093 34 with partition(x_warp, offset = thread_id, dimension = thread[1]) as x_thread:
2094 35 with partition(x_shmem_warp, offset = thread_id, dimension = thread[1]) as x_shmem_thread:
2095 36 with group(thread[1]):
2096 37 val : uint32_t @ thread[1] = x_thread[0]
2097 38
2098 39 stride : uint32_t @ thread[1] = 1
2099 40 while stride < 32:
2100 41 received : uint32_t @ thread[1] = shfl_up_sync_wrapper(val, stride)
2101 42 if thread_id >= stride:
2102 43 val = received + val
2103 44 stride *= 2
2104 45 x_shmem_thread[0] = val
2105 46
2106 47 @prism("device")
2107 48 @requires(block[1], warp[16])
2108 49 def get_warp_ends_inclusive(x : ptr(uint32_t) @ block[1], warp_ends : ptr(uint32_t) @ block[1]):
2109 50 with group(block[1]):
2110 51 warp_id : uint32_t @ warp[1] = id()
2111 52 with partition(x, offset = (warp_id * 32 * 32, dimension = warp[1]) as x_warp:
2112 53 with partition(warp_ends, offset = (warp_id * 32, dimension = warp[1]) as warp_ends_warp:
2113 54 with group(warp[1]):
2114 55 thread_id : uint32_t @ thread[1] = id()
2115 56 with partition(x_warp, offset = thread_id * 32, dimension = thread[1]) as x_thread:
2116 57 with partition(warp_ends_warp, offset = thread_id, dimension = thread[1]) as warp_ends_thread:
2117 58 with group(thread[1]):
2118 59 warp_ends_thread[0] = x_thread[31]
2119 60
2120 61
2121 62
2122 63
2123 64 @prism("device")
2124 65 @requires(block[1], warp[16])
2125 66 def update_with_new_data_and_writeback(x : ptr(uint32_t) @ block[1], x_shmem : ptr(uint32_t) @ block[1], warp_ends : ptr(uint32_t) @
2126 67 ↪ block[1], prefix : uint32_t @ block[1]):
2127 68 with group(block[1]):
2128 69 for i in range(0, (8192 * 2) / (16 * 32)):
2129 70 warp_id : uint32_t @ warp[1] = id()
2130 71 with partition(x, offset = (warp_id + i * 16) * 32, dimension = warp[1]) as x_warp:
2131 72 with partition(x_shmem, offset = (warp_id + i * 16) * 32, dimension = warp[1]) as x_shmem_warp:
2132 73 with group(warp[1]):
2133 74 thread_id : uint32_t @ thread[1] = id()
2134 75 with partition(x_warp, offset = thread_id, dimension = thread[1]) as x_thread:
2135 76 with partition(x_shmem_warp, offset = thread_id, dimension = thread[1]) as x_shmem_thread:
2136 77 with group(thread[1]):
2137 78 if warp_id + i * 16 == 0:
2138 79 x_thread[0] = prefix + x_shmem_thread[0]
2139 80 else:
2140 81 x_thread[0] = prefix + warp_ends[warp_id + i * 16 - 1] + x_shmem_thread[0]
2141 82
2142 83
2143 84
2144 85
2145 86
2146 87
2147 88
2148 89
2149 90
2150 91
2151 92
2152 93
2153 94
2154 95
2155 96
2156 97
2157 98
2158 99
2159 100

```

```

2108 @prism("device")
2109 @requires(block[1], warp[16])
2110 def naive_scan_warp_ends(x : ptr(uint32_t) @ block[1], x_buf : ptr(uint32_t) @ block[1]):
2111     with group(block[1]):
2112         stride : uint32_t @ group[1] = 1
2113         while stride < (8192 * 2 / 32):
2114             warp_id : uint32_t @ warp[1] = id()
2115             with partition(x, offset = warp_id * 32, dimension = warp[1]) as x_warp:
2116                 with partition(x_buf, offset = warp_id * 32, dimension = warp[1]) as x_buf_warp:
2117                     with group(warp[1]):
2118                         thread_id : uint32_t @ thread[1] = id()
2119                         with partition(x_warp, offset = thread_id, dimension = thread[1]) as x_thread:
2120                             with partition(x_buf_warp, offset = thread_id, dimension = thread[1]) as x_buf_thread:
2121                                 with group(thread[1]):
2122                                     if thread_id + warp_id * 32 >= stride:
2123                                         x_buf_thread[0] = x_thread[0] + x_thread[-stride]
2124                                     else:
2125                                         x_buf_thread[0] = x_thread[0]
2126             tmp : ptr(uint32_t) @ block[1] = x
2127             x = x_buf
2128             x_buf = tmp
2129             stride *= 2
2130         return x
2131
2132 # Implemented in raw CUDA: only exposing the necessary interfaces
2133 @prism("device")
2134 @requires(block[1], thread[1])
2135 def write_block_aggregate(aggregate : uint32_t @ block[1], block_idx : uint32_t @ block[1], block_infos : ptr(int) @ block[1]):
2136     pass
2137
2138 @prism("device")
2139 @requires(block[1], thread[1])
2140 def write_block_prefix(prefix : uint32_t @ block[1], block_idx : uint32_t @ block[1], block_infos : ptr(int) @ block[1]):
2141     pass
2142
2143 @prism("device")
2144 @requires(block[1], thread[1])
2145 def lookback_to_prev_blocks(block_idx : uint32_t @ block[1], block_infos : ptr(int) @ block[1]):
2146     pass
2147
2148 @prism("device")
2149 @requires(grid[1])
2150 def get_block_idx_from_global_counter(block_idx_counter : ptr(uint32_t) @ grid[1]):
2151     pass
2152
2153 @prism("global")
2154 @requires(grid[1], block[1], warp[16], smem=69632)
2155 def scan_kernel(n : uint32_t @ grid[1], x : ptr(uint32_t) @ grid[1], block_idx_counter : ptr(uint32_t) @ grid[1], block_infos :
2156     ptr(int) @ grid[1]):
2157     block_idx : uint32_t @ grid[1] = get_block_idx_from_global_counter(block_idx_counter)
2158
2159     with partition(x, offset = (8192 * 2) * block_idx, dimension = block[1]) as x_block:
2160         with group(block[1]):
2161             x_shmem : shared(uint32_t[8192 * 2]) @ block[1]
2162
2163             scan_warps(x_block, x_shmem)
2164
2165             warp_ends : shared(uint32_t[512]) @ block[1]
2166             warp_ends_buf : shared(uint32_t[512]) @ block[1]
2167
2168             get_warp_ends_inclusive(x_shmem, warp_ends)
2169             warp_ends_res : ptr(uint32_t) @ block[1] = naive_scan_warp_ends(warp_ends, warp_ends_buf)
2170
2171             aggregate : uint32_t @ block[1] = warp_ends_res[512 - 1]
2172             write_block_aggregate(aggregate, block_idx, block_infos)
2173
2174             prefix : uint32_t @ block[1] = lookback_to_prev_blocks(block_idx, block_infos)
2175             write_block_prefix(aggregate + prefix, block_idx, block_infos)
2176
2177             update_with_new_data_and_writeback(x_block, x_shmem, warp_ends_res, prefix)

```

## B.4 CUB Functions

```

1 @prism("device")
2 @requires(block[1], thread[32])
3 def block_load(input : ptr(const(int)) @ block[1],
4               output : ptr(int) @ thread[1],
5               items_per_thread : int @ block[1]):
6     with group(block[1]):
7         tid : int @ thread[32] = id()
8         with partition(input, dimension=thread[32], offset = tid * items_per_thread) as input_thrd:
9             with group(thread[32]):
10                 warp_load(input_thrd, output, items_per_thread)
11
12     return

```

```

1 @prism("device")
2 @requires(thread[32])
3 def warp_load(input : ptr(const(int)) @ thread[32],
4               output : ptr(int) @ thread[1],
5               items_per_thread : int @ thread[32]):
6     with group(thread[32]):
7         tid : int @ thread[1] = id()
8         with partition(input, dimension=thread[1], offset = tid * items_per_thread) as input_thrd:
9             with group(thread[1]):
10                 thread_load(input_thrd, output, items_per_thread)
11
12     return

```

```

1 @prism("device")
2 @requires(thread[1])
3 def thread_load(input : ptr(const(int)) @ thread[1],
4                 output : ptr(int) @ thread[1],
5                 items_per_thread : int @ thread[1]):
6     with group(thread[1]):
7         for i in range(0, items_per_thread, 1):
8             output[i] = input[i]
9     return

```

```

1 @prism("device")
2 @requires(block[1], thread[32])
3 def block_store(input : ptr(const(int)) @ thread[1],
4                 output : ptr(int) @ block[1],
5                 items_per_thread : int @ block[1]):
6     with group(block[1]):
7         tid : int @ thread[32] = id()
8         with partition(output, dimension=thread[32], offset = tid * items_per_thread) as output_thrd:
9             with group(thread[32]):
10                 warp_store(input, output_thrd, items_per_thread)
11
12     return

```

```

1 @prism("device")
2 @requires(thread[32])
3 def warp_store(input : ptr(const(int)) @ thread[1],
4                output : ptr(int) @ thread[32],
5                items_per_thread : int @ thread[32]):
6     with group(thread[32]):
7         tid : int @ thread[1] = id()
8         with partition(output, dimension=thread[1], offset = tid * items_per_thread) as output_thrd:
9             with group(thread[1]):
10                 thread_store(input, output_thrd, items_per_thread)
11
12     return

```

```

1 @prism("device")
2 @requires(thread[1])
3 def thread_store(input : ptr(const(int)) @ thread[1],
4                  output : ptr(int) @ thread[1],
5                  items_per_thread : int @ thread[1]):
6     with group(thread[1]):
7         for i in range(0, items_per_thread, 1):
8             output[i] = input[i]
9     return

```

## B.5 H100 Matrix Multiplication

2206

2207

2208

2209

2210

2211

2212

2213

2214

2215

2216

2217

2218

2219

2220

2221

2222

2223

2224

2225

2226

2227

2228

2229

2230

2231

2232

2233

2234

2235

2236

2237

2238

2239

2240

2241

2242

2243

2244

2245

2246

2247

2248

2249

2250

2251

2252

2253

2254

```

1 @prism("global")
2 @attr("__launch_bounds__(128*3)")
3 @requires(grid[1], block[1], warp[12], smem=227000)
4 def my_h100_match_no_tail(
5     M: int @ grid[1],
6     N: int @ grid[1],
7     K: int @ grid[1],
8     C: ptr(bf16) @ grid[1],
9     tensorMapA: const(CUtensorMap) @ grid[1],
10    tensorMapB: const(CUtensorMap) @ grid[1]):
11
12    with group(grid[1]):
13        BM : constexpr(int) @ grid[1] = 128
14        BN : constexpr(int) @ grid[1] = 256
15        BK : constexpr(int) @ grid[1] = 64
16        NUM_THREADS : constexpr(int) @ grid[1] = 128*3
17        QSIZE : constexpr(int) @ grid[1] = 4
18        NUM_SM : constexpr(int) @ grid[1] = 128
19
20        WGMMMA_M : constexpr(int) @ grid[1] = 64
21        WGMMMA_K : constexpr(int) @ grid[1] = 16
22        WGMMMA_N : constexpr(int) @ grid[1] = BN
23        num_consumers : constexpr(int) @ grid[1] = (NUM_THREADS / 128) - 1
24        B_WG_M : constexpr(int) @ grid[1] = BM / num_consumers
25
26        TM : constexpr(int) @ grid[1] = 16
27        TN : constexpr(int) @ grid[1] = 8
28        schedule_block : int @ block[1] = id()
29
30        with partition(C, offset=0, dimension=block[1]) as block_C:
31            with group(block[1]):
32
33                # Allocate SA
34                # sA[QSIZE][BK*BM]
35                sA_slot0 : shared(bf16[64* 128], align=128) @ block[1]
36                sA_slot1 : shared(bf16[64* 128]) @ block[1]
37                sA_slot2 : shared(bf16[64* 128]) @ block[1]
38                sA_slot3 : shared(bf16[64* 128]) @ block[1]
39
40                # Allocate SB
41                # sB[QSIZE][BK*BN]
42                sB_slot0 : shared(bf16[64* 256], align=128) @ block[1]
43                sB_slot1 : shared(bf16[64* 256]) @ block[1]
44                sB_slot2 : shared(bf16[64* 256]) @ block[1]
45                sB_slot3 : shared(bf16[64* 256]) @ block[1]
46
47                num_blocks_k : const(int) @ block[1] = K / BK
48                wg_idx : int @ warp[4] = id()
49                blk_thrd_id : int @ thread[1] = id()
50
51
52                tid : int @ thread[1] = id() % 128
53                is_producer : bool @ warp[4] = wg_idx == 0
54
55                num_block_m : int @ block[1] = 0
56                num_block_n : int @ block[1] = 0
57
58                with group(warp[4]):
59                    if (is_producer):
60                        pass
61                    else:
62                        wg_idx = wg_idx - 1
63
64                schedule_it : int @ block[1] = 0
65                total_blocks_m : int @ block[1] = (((M + BM) - 1) / BM)
66                total_blocks_n : int @ block[1] = (((N + BN) - 1) / BN)
67                unsafe("assert((CEIL_DIV(M, BM)%TM == 0 && total_blocks_n%TN == 0));")
68
69                while(true):
70                    num : int @ block[1] = ((schedule_it * NUM_SM) + schedule_block)
71                    if (num >= (total_blocks_m * total_blocks_n)):
72                        break
73                    cur_tile : int @ block[1] = (num / (TM * TN))
74                    cur_tile_pos : int @ block[1] = (num % (TM * TN))
75                    num_block_m = TM * (cur_tile / (total_blocks_n / TN))
76                    num_block_n = TN * (cur_tile % (total_blocks_n / TN))
77                    num_block_m += (cur_tile_pos / TN)
78                    num_block_n += (cur_tile_pos % TN)
79                    schedule_it += 1
80                    d : c_float[1][16][8] @ thread[1]
81
82

```

2303



```

2304 165         for k_it in range(0, 64/WGMMMA_K, 1):
2305 166             intrinsic.wgmma256(sa_1_producer[64*(m_it + wg_idx*B_WG_M/WGMMMA_M)*WGMMMA_M
                ↳ + index_a2 + k_it*WGMMMA_K], sb_1_producer[(index_b2 + (k_it *
2306 167                 ↳ WGMMMA_K))], 1, 1, 1, 0, 0, out=[d[m_it]])
2307 168
2308 169         with wgmma_async():
2309 170             for m_it in range(0, B_WG_M/WGMMMA_M, 1):
2310 171                 index_a3 : int @ warp[4] = m_it * BM
2311 172                 index_b3 : int @ warp[4] = m_it * BN
2312 173                 unsafe("#pragma unroll")
2313 174                 for k_it in range(0, 64/WGMMMA_K, 1):
2314 175                     intrinsic.wgmma256(sa_2_producer[64*(m_it + wg_idx*B_WG_M/WGMMMA_M)*WGMMMA_M
2315 176                         ↳ + index_a3 + k_it*WGMMMA_K], sb_2_producer[(index_b3 + (k_it *
2316 177                             ↳ WGMMMA_K))], 1, 1, 1, 0, 0, out=[d[m_it]])
2317 178
2318 179         with wgmma_async():
2319 180             for m_it in range(0, B_WG_M/WGMMMA_M, 1):
2320 181                 index_a4 : int @ warp[4] = m_it * BM
2321 182                 index_b4 : int @ warp[4] = m_it * BN
2322 183                 unsafe("#pragma unroll")
2323 184                 for k_it in range(0, 64/WGMMMA_K, 1):
2324 185                     intrinsic.wgmma256(sa_3_producer[64*(m_it + wg_idx*B_WG_M/WGMMMA_M)*WGMMMA_M
2325 186                         ↳ + index_a4 + k_it*WGMMMA_K], sb_3_producer[(index_b4 + (k_it *
2326 187                             ↳ WGMMMA_K))], 1, 1, 1, 0, 0, out=[d[m_it]])
2327 188
2328 189         case 4:
2329 190             pass
2330 191
2331 192     with claim(block_C, scope=warp[8], offset=num_block_n*BN*M + num_block_m*BM) as c_consumer:
2332 193         match warp:
2333 194             case 8:
2334 195                 with partition(c_consumer, dimension=thread[1], offset=0) as c_thrd:
2335 196                     with group(warp[4]):
2336 197                         warp_id: int @ warp[1] = id()
2337 198                         with group(warp[1]):
2338 199                             lane : int @ thread[1] = id()
2339 200                             row : int @ thread[1] = warp_id * 16 + lane / 4
2340 201                             unsafe("#pragma unroll")
2341 202                             for m_it in range(0, B_WG_M/WGMMMA_M, 1):
2342 203                                 yo : int @ warp[1] = m_it*WGMMMA_M + wg_idx*B_WG_M
2343 204                                 with group(thread[1]):
2344 205                                     if (row + yo + num_block_m*BM >= M):
2345 206                                         continue
2346 207                                     for w in range(0, WGMMMA_N, 16):
2347 208                                         if (w < w < N-num_block_n*BN):
2348 209                                             col : int @ thread[1] = w + 2*(tid % 4);
2349 210                                             c_thrd[col * M + row + yo] = d[m_it][w/16][0]
2350 211                                             c_thrd[(col + 1) * M + (row + yo)] = d[m_it][w/16][1]
2351 212                                             c_thrd[(col + 1) * M + (row + 8) + yo] = d[m_it][w/16][2]
2352 213                                             c_thrd[(col + 1) * M + (row + 8) + yo] = d[m_it][w/16][3]
2353 214
2354 215                                             c_thrd[(col + 8) * M + (row + 0) + yo] = d[m_it][w/16][4]
2355 216                                             c_thrd[(col + 9) * M + (row + 0) + yo] = d[m_it][w/16][5]
2356 217                                             c_thrd[(col + 8) * M + (row + 8) + yo] = d[m_it][w/16][6]
2357 218                                             c_thrd[(col + 9) * M + (row + 8) + yo] = d[m_it][w/16][7]
2358 219
2359 220             case 4:
2360 221                 pass
2361 222
2362 223     return

```
